# Supplementary material for: SGOOD: Substructure-enhanced Graph-Level Out-of-Distribution Detection
Source: arXiv:2310.10237 source file (2024-07-18)
Supplement: Supplementary file 1 [file appendix.tex]

\newpage
\appendix
\onecolumn
\section*{Appendix}

We provide the proof of Proposition \ref{prop:power} in Appendix \ref{apx:proof}, more experimental details on datasets, evaluation metrics, implementation in Appendix \ref{apx:setup},  several additional experiments for effectiveness, efficiency and visualization in Appendix \ref{apx:exp}, and the pseudo code of \algo in Appendix \ref{apx:algo}.

\section{Proof for Proposition~\ref{prop:power}}\label{apx:proof}

\begin{proof}
We first prove that \algo is at least as powerful as 1\&2-WL in Lemma \ref{lm:1}. Then, we prove that \algo can distinguish 2-regular graphs that 1\&2-WL cannot distinguish in Lemma \ref{lm:2}. Combining these two Lemmas, we prove that \algo is strictly more powerful than  1\&2-WL.

%In summary, Lemma \ref{lm:1} indicates that \algo is at least as powerful as 1\&2-WL. Lemma \ref{lm:2} further indicates that \algo can distinguish 2-regular graphs that 1\&2-WL can not. 
%By combining the results from Lemma \ref{lm:1} and Lemma \ref{lm:2}, we have successfully proven Proposition~\ref{prop:power} that \algo is strictly more powerful than 1\&2-WL. 
\end{proof}

% ************************Lemma 1************************************

\begin{lemma}\label{lm:1}
Let $G_1=(V_1, E_1)$ and $G_2=(V_2, E_2)$ be two graphs identified as non-isomorphic by  1\&2-WL. 
\algo projects them into  different representations $\mathbf{h}_{\mathcal{G}_1}$ and $\mathbf{h}_{\mathcal{G}_2}$ in Eq. \eqref{eq:sub_pool}.
\end{lemma}
\begin{proof}
Let $\mathcal{H}_{1}^{G}=\{\mathbf{h}_{v}|v\in {V}_{1} \}$ and $\mathcal{H}_{2}^{G}=\{\mathbf{h}_{v}|v\in {V}_{2} \}$ be the  multisets of node representations of $G_1$ and $G_2$ generated by GIN in Eq. \eqref{eq:node_pool}, respectively. Let $\mathcal{G}_1=(\mathcal{V}_{1}, \mathcal{E}_{1})$ and $\mathcal{G}_2=(\mathcal{V}_{2}, \mathcal{E}_{2})$ be the super graphs of $G_1$ and $G_2$ respectively.  We consider two cases: (1) $|\mathcal{V}_{1}| \neq |\mathcal{V}_{2}|$, (2) $|\mathcal{V}_{1}| = |\mathcal{V}_{2}|$.

For case (1), $\mathcal{G}_1$ and $\mathcal{G}_2$ are two graphs with different number of nodes. Thus, $\mathcal{G}_1$ and $\mathcal{G}_2$ can be easily determined as non-isomorphic by 1\&2-WL. It is  proved that GIN with sufficient number of layers and all injective functions is as powerful as 1\&2-WL \citep{xu2018powerful}. As GIN is adopted in \algo as GNN backbone  with sufficient number of layers and $\texttt{\small{READOUT}}$ function in Eq.\eqref{eq:sub_pool} is injective,    representations $\mathbf{h}_{\mathcal{G}_1}$ and 
$\mathbf{h}_{\mathcal{G}_2}$of  $\mathcal{G}_1$ and $\mathcal{G}_2$ are different.

For case (2), let $|\mathcal{V}_{1}| = |\mathcal{V}_{2}| = K$. Let $\mathcal{H}_{1}^{\mathcal{G}}= \{\mathbf{h}^{(0)}_{g_{1,j}}|g_{1,j}\in \mathcal{V}_{1}\}$ and $\mathcal{H}_{2}^{\mathcal{G}}= \{\mathbf{h}^{(0)}_{g_{2,j}}|g_{2,j}\in \mathcal{V}_{2}\}$ be the multisets of initial node representations of $\mathcal{G}_1$ and $\mathcal{G}_2$ calculated by Eq.\eqref{eq:node_pool}, respectively. 
Using GIN with sufficient number of layers, we have $\mathcal{H}_{1}^{G} \neq \mathcal{H}_{2}^{G}$ \citep{xu2018powerful}. As stated in Section \ref{sec::substructure}, the substructures $\{\subij\}_{j=1}^{n_{i}}$ of a graph $G_i$ satisfy the following properties: (i) the substructures are non-overlapping, (ii) the union of the nodes in all substructures is the node set of $G_i$. Thus, $\{\{\mathbf{h}_{v}|v\in {g}_{1,j}\}\}_{j=1}^{K}$ (resp. $\{\{\mathbf{h}_{v}|v\in {g}_{2,j}\}\}_{j=1}^{K}$) is a partition of $\mathcal{H}_{1}^{G}$ (resp. $\mathcal{H}_{2}^{G}$). Then, we have
$\{\{\mathbf{h}_{v}|v\in {g}_{1,j}\}\}_{j=1}^{K} \neq \{\{\mathbf{h}_{v}|v\in {g}_{2,j}\}\}_{j=1}^{K}$. As $\texttt{\small{POOL}}$ function in Eq.\eqref{eq:node_pool} is injective, we have $\{\texttt{\small{POOL}}(\{\mathbf{h}_{v}|v\in {g}_{1,j}\})\}_{j=1}^{K} \neq \{\texttt{\small{POOL}}(\{\mathbf{h}_{v}|v\in {g}_{2,j}\})\}_{j=1}^{K}$, that is $\mathcal{H}_{1}^{\mathcal{G}} \neq \mathcal{H}_{2}^{\mathcal{G}}$. As GIN with sufficient number of layers  and $\texttt{\small{READOUT}}$ function in Eq.\eqref{eq:sub_pool} are both injective, we derive that representations $\mathbf{h}_{\mathcal{G}_1}$ and 
$\mathbf{h}_{\mathcal{G}_2}$ generated on  $\mathcal{H}_{1}^{\mathcal{G}}$ and $\mathcal{H}_{2}^{\mathcal{G}}$ are different.

Combining case (1) and case (2), we prove Lemma \ref{lm:1}.
\end{proof}

Next, we   prove that  \algo can distinguish 2-regular graphs that 1\&2-WL cannot distinguish in Lemma \ref{lm:2}. Before that, we first give the definition of 2-regular graphs. Note that we only consider undirected graphs in this paper.
\begin{definition}[2-regular graph] A graph is said to be regular of degree 2 if all local degrees are  2. 
\end{definition}
Based on the definition of a 2-regular graph, we can conclude that   a 2-regular graph consists of one or more (disconnected) cycles.
% ************************Lemma 2************************************
\begin{lemma}\label{lm:2}
Given two non-isomorphic $n$-node 2-regular graphs $G_1=(V_1, E_1)$ and $G_2=(V_2, E_2)$ that 1\&2-WL cannot distinguish, \algo projects them into  different graph representations $\mathbf{h}_{\mathcal{G}_1}$ and $\mathbf{h}_{\mathcal{G}_2}$in Eq. \eqref{eq:sub_pool}.
\end{lemma}
\begin{proof}

%  We consider two cases: (1) $|\mathcal{V}_{1}| \neq |\mathcal{V}_{2}|$, (2) $|\mathcal{V}_{1}| = |\mathcal{V}_{2}|$.
 
% For case (1), $\mathcal{G}_1$ and $\mathcal{G}_2$ are two graphs with different number of nodes. Thus, $\mathcal{G}_1$ and $\mathcal{G}_2$ can be easily determined as non-isomorphic by 1\&2-WL. Xu \etal\citep{xu2018powerful} proved that GIN with sufficient number of layers and all injective functions is as powerful as 1\&2-WL. As  GNNs adopted in \algo are GIN with sufficient number of layers and $\texttt{\small{READOUT}}$ function in Eq.\eqref{eq:sub_pool} is injective,  graph representations $\mathbf{h}_{\mathcal{G}_1}$ and 
% $\mathbf{h}_{\mathcal{G}_2}$ generated on  $\mathcal{G}_1$ and $\mathcal{G}_2$ are different.

% For case (2), let $|\mathcal{V}_{1}| = |\mathcal{V}_{2}| = K>1$. 

Based on the definition of a 2-regular graph, we can say that  $G_1$ and $G_2$  consist of one or more disconnected cycles. Let $r_1$ and $r_2$ be the number of cycles in  $G_1$ and $G_2$, respectively. We consider two cases: (1) $r_1 \neq 1  \wedge
 r_2 \neq 1$, (2) $(r_1=1 \wedge r_2\neq 1)\vee(r_1\neq1 \wedge r_2= 1)$.
 
For case (1), $G_1$ and $G_2$ consist of disconnected circles.  Let $\mathcal{G}_1=(\mathcal{V}_{1}, \mathcal{E}_{1})$ and $\mathcal{G}_2=(\mathcal{V}_{2}, \mathcal{E}_{2})$ be the constructed super graphs of $G_1$ and $G_2$, respectively.  $\mathcal{G}_1$ and $\mathcal{G}_2$ are constructed by modularity-based community detection method \citep{clauset2004finding} that assign nodes in a graph to different clusters when the
 modularity of the graph is maximized under such cluster assignment.
As \citet{brandes2007modularity} proves in Lemma 3.4,  there is always a clustering with maximum
modularity, in which each cluster consists of a connected
subgraph. As a result, $\forall g_{1,j} \in \mathcal{V}_{1}$ is a circle in $G_1$, and $|\mathcal{V}_{1}|=r_1$. Similarly,  $\forall g_{2,j} \in \mathcal{V}_{2}$ is  a circle in $G_2$, and $|\mathcal{V}_{2}|=r_2$. Let $\mathcal{N}_{1} = \{|V_{1,j}|\}_{j=1}^{|\mathcal{V}_{1}|}$ and $\mathcal{N}_{2} = \{|V_{2,j}|\}_{j=1}^{|\mathcal{V}_{2}|}$.
Since $G_1$ and $G_2$ are non-isomorphic, we have $\exists n_{1,j} \in \mathcal{N}_{1}: \forall n_{2,j} \in \mathcal{N}_{2}, n_{1,j} \neq n_{2,j}$. As a result, we have $\mathcal{N}_{1} \neq \mathcal{N}_{2}$. Then, we have
$\{\{\mathbf{h}_{v}|v\in {V}_{1,j}\}\}_{j=1}^{|\mathcal{V}_{1}|} \neq \{\{\mathbf{h}_{v}|v\in {V}_{2,j}\}\}_{j=1}^{|\mathcal{V}_{2}|}$. As $\texttt{\small{POOL}}$ function in Eq.\eqref{eq:node_pool} is injective, we have $\{\texttt{\small{POOL}}(\{\mathbf{h}_{v}|v\in {g}_{1,j}\})\}_{j=1}^{|\mathcal{V}_{1}|} \neq \{\texttt{\small{POOL}}(\{\mathbf{h}_{v}|v\in {g}_{2,j}\})\}_{j=1}^{|\mathcal{V}_{2}|}$, that is $\mathcal{H}_{1}^{\mathcal{G}} \neq \mathcal{H}_{2}^{\mathcal{G}}$. As GIN with sufficient number of layers  and $\texttt{\small{READOUT}}$ function in Eq.\eqref{eq:sub_pool} are both injective, we have  representations $\mathbf{h}_{\mathcal{G}_1}$ and 
$\mathbf{h}_{\mathcal{G}_2}$ generated on  $\mathcal{H}_{1}^{\mathcal{G}}$ and $\mathcal{H}_{2}^{\mathcal{G}}$ are different.

For case (2), we consider $r_1=1 \wedge r_2\neq 1$, and the proof when $r_2=1 \wedge r_1\neq 1$  is similar. $G_1$  consists of one single circle, and $G_2$  consists of $r_2$ disconnected circles.  Let $\mathcal{G}_1=(\mathcal{V}_{1}, \mathcal{E}_{1})$ and $\mathcal{G}_2=(\mathcal{V}_{2}, \mathcal{E}_{2})$ be the constructed super graphs of $G_1$ and $G_2$, respectively. For $G_2$ and $\mathcal{G}_2$, $\forall g_{2,j} \in \mathcal{V}_{2}$ is  a circle in $G_2$, and $|\mathcal{V}_{2}|=r_2$
following the conclusion in case (1). For $G_1$ and $\mathcal{G}_1$, we consider two cases: (i) $|\mathcal{V}_{1}|=r_1=1$, and (ii) $|\mathcal{V}_{1}|>1$. For case (i), $\mathcal{V}_{1}=\{g_{1,1}\}$, where $g_{1,1}=G_1$. Let $\mathcal{N}_{1} = \{|V_{1,j}|\}_{j=1}^{|\mathcal{V}_{1}|}=\{|V_{1,1}|\}$ and $\mathcal{N}_{2} = \{|V_{2,j}|\}_{j=1}^{|\mathcal{V}_{2}|}$, where $|\mathcal{V}_{2}|>1$. We have $\mathcal{N}_{1} \neq \mathcal{N}_{2}$. Similar to case (1), we have the same conclusion that graph representations $\mathbf{h}_{\mathcal{G}_1}$ and 
$\mathbf{h}_{\mathcal{G}_2}$ generated on  $\mathcal{H}_{1}^{\mathcal{G}}$ and $\mathcal{H}_{2}^{\mathcal{G}}$ are different. For case (ii), $\mathcal{V}_{1}=\{g_{1,j}\}_{j=1}^{|\mathcal{V}_{1}|}$, where $\forall g_{1,j} \in \mathcal{V}_{1}$ is a chain and two nearby chain are connected in $\mathcal{G}_1$. In other words, $\mathcal{G}_1$ is a $|\mathcal{V}_{1}|$-circle while $\mathcal{G}_2$ consists of $|\mathcal{V}_{2}|$ isolated nodes. Thus, $\mathcal{G}_1$ and $\mathcal{G}_2$ can be easily distinguished as non-isomorphic by 1\&2-WL.  According to \citep{xu2018powerful}, when we encode $\mathcal{G}_1$ and $\mathcal{G}_2$ by Eq. \eqref{eq:sub_mp} with sufficient layers of GIN, and generate  $\mathbf{h}_{\mathcal{G}_1}$ and 
$\mathbf{h}_{\mathcal{G}_2}$ by   Eq. \eqref{eq:sub_pool}, where $\texttt{\small{READOUT}}$ is injective, $\mathbf{h}_{\mathcal{G}_1}$ and 
$\mathbf{h}_{\mathcal{G}_2}$ are different. Combining case (i) and case (ii), we prove that \algo generates different $\mathbf{h}_{\mathcal{G}_1}$ and 
$\mathbf{h}_{\mathcal{G}_2}$ for $G_1$ and $G_2$ in case (2).

Combining  case (1) and case (2), we prove Lemma \ref{lm:2}.
\end{proof}

% $G_1$ and $G_2$ satisfy one of the following properties: 

% (i) $G_1$ and $G_2$ consist of different number of circles, and  $|\mathcal{N}_{1}| \neq |\mathcal{N}_{2}|$, (ii) $G_1$ and $G_2$ consist of the same  number of circles, but .

\section{Experimental Settings}\label{apx:setup}
We provide more details on datasets, evaluation metrics, and implementation here for reproducibility.
All experiments are conducted on a Linux server with Intel Xeon Gold 6226R 2.90GHz CPU and an Nvidia RTX 3090 GPU card.

\subsection{Dataset Details}\label{apx::datasets}
We adopt  real-world datasets in various data domains for graph-level OOD detection. The dataset statistics is listed in Table \ref{tab:datasets}. Following  existing work \citep{liu2023good, li2022graphde}, given a graph dataset, we use graphs of the same type with distribution shift as ID and OOD data, respectively. The detailed descriptions of ID and OOD graphs in the 6 datasets are as follows.  
\begin{itemize}[leftmargin=*]
    \item \textbf{\enzymes}\citep{morris2020tudataset} dataset comprises protein networks representing enzymes classified into 6 EC top-level classes. In this paper, we consider graphs from \emph{all} classes in \enzymes as in-distribution (ID) graphs. To introduce OOD graphs, we utilize graphs from the PROTEINS dataset \citep{morris2020tudataset}. PROTEINS is also a dataset of protein networks, where graphs are labeled as either 'Enzymes' or 'Non-enzymes'. Specifically, we use graphs in PROTEINS with label 'Non-enzymes' as OOD graphs. Consequently, the OOD graphs in \enzymes represent unseen classes.
    
    \item \textbf{\multi} \citep{morris2020tudataset} is a dataset of social networks. It consists of ego-networks derived from actor collaborations. The graphs are labeled with three genres: Comedy, Romance, and Sci-Fi. 
    We consider graphs from \emph{all} classes in \multi as ID graphs.
    To introduce OOD graphs, we utilize graphs from another dataset called \binary \citep{morris2020tudataset}. Similar to \multi, \binary is also a dataset of social networks, but the graphs are labeled as either 'Action' or 'Romance'. Specifically, we use graphs labeled as 'Action' as OOD graphs. These OOD graphs do not belong to any classes in \multi, and they represent unseen classes.

    \item \textbf{\binary} \citep{morris2020tudataset} dataset is constructed in a similar manner to \multi. Specifically, we consider graphs from \emph{both} classes (Action and Romance) in \binary as ID graphs. On the other hand, we regard graphs labeled as 'Comedy' or 'Sci-Fi' in \multi as OOD graphs. These OOD graphs represent classes that are not present in \binary, and they are with unseen classes.
    
    \item \textbf{\reddit} \citep{yanardag2015deep} dataset is a large-scale dataset of social networks. It consists of graphs corresponding to an online discussion thread in REDDIT where nodes correspond to users. The graphs are labeled as 11 classes based on the subreddit they belong to. In this paper, we consider graphs from \emph{all} classes in \reddit as in-distribution (ID) graphs. To introduce OOD graphs, we utilize graphs from the REDDIT-BINARY dataset \citep{yanardag2015deep} where graphs  also represents online discussion threads and are labeled as question/answer-based community or a discussion-based community. 
    Consequently, the OOD graphs in \reddit represent unseen classes.

    \item \textbf{\bace} \citep{wu2018moleculenet} is a dataset of molecular graphs used for predicting particular physiology properties of chemical compounds. The dataset is split into  training/validation/test sets based on the scaffolds of molecules. Notably, the samples in the training set have distinct scaffolds compared to those in the validation and test sets.  The molecular properties of different scaffolds are often quite different~\citep{ji2022drugood}. We consider graphs from the training set as ID graphs, while graphs from the test set are treated as OOD graphs. The OOD graphs exhibit a scaffold distribution that differs from   ID graphs.
    
    \item \textbf{\bbbp} \citep{wu2018moleculenet} is   a dataset of molecular graphs for predicting barrier permeability. Like  \bace dataset, \bbbp is split into training, validation, and test sets based on the scaffolds of molecules. We consider graphs from the training set as ID graphs, while graphs from the test set are treated as OOD graphs. The OOD graphs exhibit a scaffold distribution that differs from  the ID graphs.

    \item \textbf{\drug} is a dataset of molecular graphs generated by the dataset curator provided by \citep{ji2022drugood}, which is a systematic OOD dataset curator and benchmark for AI-aided drug discovery. We  focus on the sub-dataset DrugOOD-sbap-core-ec50-protein, which contains molecular graphs for the task structure-based affinity prediction.  The dataset is split into  training/validation/test sets based on the protein target of molecules. Graphs from the training set are considered ID graphs, while graphs from the test set are treated as OOD graphs. The OOD graphs exhibit a protein target distribution that differs from that of the ID graphs.
     \item \textbf{\hiv} \citep{wu2018moleculenet} is   a large-scale dataset of molecular graphs for testing compounds on the ability to inhibit HIV replication. Like  \bace and \bbbp dataset, \hiv is split into training, validation, and test sets based on the scaffolds of molecules. We consider graphs from the training set as ID graphs, while graphs from the test set are treated as OOD graphs. The OOD graphs exhibit a scaffold distribution that differs from  the ID graphs.  
    % \item \textbf{DrugOOD-Scaffold}
    % is a dataset of molecular graphs generated by the dataset curator provided by DrugOOD\citep{ji2022drugood}. Specially, molecules  are split into  training/validation/test sets according to their scaffold. We use the training set as ID graphs and test set as OOD graphs. 
\end{itemize}

\subsection{Evaluation Metrics}\label{apx::metrics}
We explain in details the OOD detection evaluation metrics.  We use three commonly-used metrics \auc, \pr and \fpr for OOD detection evaluation \citep{hendrycks2016baseline,wu2023energy}. All the three metrics are independent of threshold choosing. 
\begin{itemize}[leftmargin=*]
    \item \textbf{\auc}, short for Area Under the Receiver Operating Characteristic (ROC) Curve, is a widely used performance metric. It quantifies the area under the ROC curve, which plots the True Positive Rate (TPR) against the False Positive Rate (FPR) across different probability thresholds ranging from 0 to 1. The \auc score provides a comprehensive assessment of a model's ability to differentiate between the positive and negative classes, reflecting its overall discriminative power.
    
    \item \textbf{\pr} stands for Area Under the Precision-Recall Curve. Precision-Recall curve is a plot of precision versus recall at various probability thresholds ranging from 0 to 1. Higher \pr indicates that positive samples are correctly identified while false positive predictions are minimized. \pr is particularly useful in imbalanced datasets where one class is significantly underrepresented compared to the other.%, while \auc is sensitive to class imbalance. 
    
    \item \textbf{\fpr} stands for False Positive Rate at 95\% True Positive Rate.  \fpr measures the false positive rate (FPR) when the true positive rate (TPR) is 95\%. A lower \fpr value indicates better performance, as it means the classifier is able to maintain a high true positive rate while minimizing false positive predictions.
\end{itemize}

% Specially, \auc stands for Area Under the Receiver Operating Characteristic (ROC) Curve, it measures area under the ROC curve, which is a plot of the True Positive Rate (TPR) against the False Positive Rate (FPR) at various probability thresholds ranging from 0 to 1. \auc  provides an overall measure of how well the classifier can distinguish between the positive and negative classes. \pr stands for Area Under the Precision-Recall Curve. Precision-Recall curve is a plot of precision versus recall at various probability thresholds ranging from 0 to 1. Higher \pr indicates that positive samples are correctly identified while false positive predictions are minimized. \pr is particularly useful in imbalanced datasets where one class is significantly underrepresented compared to the other while \auc is more sensitive to class imbalance. 
% \fpr stands for False Positive Rate at 95\% True Positive Rate.  \fpr measures the false positive rate (FPR) when the true positive rate (TPR) is 95\%. A lower \fpr value indicates better performance, as it means the classifier is able to maintain a high true positive rate while minimizing false positive predictions.

\subsection{Implementation Details of Baselines}\label{apx::baselines}
We provide more description and implementation details of the baselines in Section~\ref{sec:experiments}.
\begin{itemize}
    \item \textbf{\msp, \energy, \odin} are general OOD detection methods that estimate OOD scores directly from classification logits at test time. Specially, \msp~\citep{hendrycks2016baseline} is the first and the most basic baseline that directly uses the maximum softmax score as OOD score. \energy~\citep{liu2020energy} uses energy function that works directly on the output logits to predict OOD scores. \odin~\citep{liang2017enhancing} uses temperature scaling with gradient-based input perturbations to enlarge the outputs  differences between OOD and ID samples.
    \item \textbf{\md}~\citep{lee2018simple} is a distance-based OOD detection method. It models the feature embedding space as a mixture of multivariate Gaussian distributions and  measures OOD scores according to the \md distance between test samples and ID training data.
    \item \textbf{\safe}~\citep{wu2023energy} is a graph OOD detection method based on energy model. It incorporates GNNs in the energy model and detects OOD samples using energy scores. For node-level OOD detection, it further adopts a propagation scheme to leverage graph structure through unlabeled nodes. In our paper, we use graph labels to directly run the basic version of \safe from its Section 3.1~\citep{wu2023energy}.
    \item \textbf{\graphde}~\citep{li2022graphde} is a graph-level OOD detection method based on probabilistic model.  It addresses both the challenges of debiased learning and OOD detection in graph data. By modeling the graph generative process and incorporating a latent environment variable, the model can automatically identify outliers during training and serve as an effective OOD detector.
    \item \textbf{\good}~\citep{liu2023good}  is an unsupervised graph-level OOD detection method. It detects OOD graphs solely based on unlabeled ID data. GOOD-D utilizes a graph contrastive learning framework combined with perturbation-free graph data augmentation to capture latent ID patterns and detect OOD graphs based on semantic inconsistency at multiple levels of granularity.
    \item \textbf{\ocgin}~\citep{zhao2021using} is a graph-level anomaly detection method that combines deep one-class classification with GIN~\citep{xu2018powerful}.  It aims to project the outlier graphs at a significant distance from the training graphs in the learned feature space.
    \item \textbf{\ocgtl}~\citep{qiu2022raising} is a graph-level anomaly detection method based on self-supervised learning and transformation learning. It develops an one-class objective that encourages graph embeddings of training data to concentrate within a hyper-sphere and outlier graphs are distant to the hyper-sphere.

    \item \textbf{\glkd}~\citep{ma2022deep} is a graph-level anomaly detection method. By training a predictor network to reproduce representations from a randomly-initialized network, the model learns both global and local normal patterns in the training data. Anomaly scores are then computed based on the prediction error, allowing the detection of irregular or abnormal graphs.
\end{itemize}

\paragraph{Implementation Details.}
For \msp, \energy, \odin, and \md baselines, we substitute the network backbone in their official implementation with a 5-layer GIN~\citep{xu2018powerful} using a fixed hidden dimension of $16$ to encode graphs into node representations.
The node representations from different layers are first concatenated and then aggregated using sum pooling for the final graph representations. Graph representations are sent to linear layer for classification logits. Other experimental settings are the same as \algo. 
For \odin, as we lack auxiliary OOD data for hyperparameter fine-tuning, we initially explore the temperature values from ${1, 10, 100, 1000}$ and the perturbation magnitudes from ${0, 0.001, 0.002, 0.004}$ on all datasets. After experimental tuning, we set the temperature to 10 and the perturbation magnitude to 0.002 consistently achieves competitive performance across all datasets. This configuration is then fixed for further evaluation.
For \md, we leverage the graph representations used for classification to compute the \md distance, which serves as the estimated OOD scores. However, we do not employ the calibration techniques, such as input pre-processing and feature ensemble in the original paper \citep{lee2018simple}. We observed a significant drop in performance when implementing \md with these techniques. We guess the reason is that the calibration techniques designed for image data are not suitable for graphs.
For the other competitors, we use their original codes provided by the respective authors. 
All competitors are trained using ID training graphs and fine-tuned using ID graphs in validation set.

% The graph transformation $\mathcal{T}_{0}$ and $\mathcal{T}_{1}$ is searched from different combination of $\mathcal{A}$ according to classification loss on the validation set. 
% The performance of \algo on test set is reported when  \algo achieves the lowest classification loss on the validation set.

% For \msp, \energy, \odin, and \md,  we replace the network backbone in the official implementation with 5-layer GIN with fixed hidden dimension $16$ to encode graphs into node representations. 
% The node representations from different layers are first concatenated and then aggregated with sum pooling for the final graph representations. Graph representations are sent to linear layer for classification logits. Other experimental settings are the same as \algo. For the other competitors, we use their original codes provided by the respective authors. 
% All competitors are trained using ID training graphs and fine-tuned using ID graphs in validation set.

% For training the competitors, the graph  augmentations are chosen from common  graph augmentations $\mathcal{A}=\{\text{Edge Perturbation},\text{Attribute Masking},\text{Node Dropping},\text{Subgraph}\}$ \citep{you2020graph, ding2022data} according to classification loss on the validation set. We set augmentation ratio as 0.2 for the competitors following GraphCL\citep{you2020graph}. The results are given in Table \ref{tab:subgraph}.

\section{Additional Experiments}\label{apx:exp}
\paragraph{Performance on ID graph classification.}
Table~\ref{tab:acc} reports the performanc on ID graph classification of all methods by Accuracy (ID ACC). We observe that \algo  achieves best ID ACC on 7/8 datasets, which indicates that leveraging substructures also benefits graph classification. 
Nevertheless, note that, as mentioned, the main goal of OOD detection is to accurately identify OOD data during testing, while maintaining instead of significantly improving ID ACC.

\begin{table}[htbp]
  \caption{ ID graph classification performance measured by  \acc.  All results are reported in percentage \% (mean ± std). {/ indicates that \acc is not applicable for  unsupervised  methods.} }
  \resizebox{\textwidth}{!}{
  \hspace{-3mm}
    \begin{tabular}{ccccccccc}
    \toprule
    \multicolumn{1}{l}{Method} & \multicolumn{1}{l}{ENZYMES} & \multicolumn{1}{l}{IMDB-M} & \multicolumn{1}{l}{IMDB-B} & \multicolumn{1}{l}{\reddit} & \multicolumn{1}{l}{BACE} & \multicolumn{1}{l}{BBBP} & \multicolumn{1}{l}{HIV} & \multicolumn{1}{l}{DrugOOD} \\
    \midrule
    MSP   & 37.33 & 48.27 & 69.80 & 48.91 & 80.83 & 87.44 & 96.62 & 79.20 \\
    Energy & 37.33 & 48.27 & 69.80 & 48.91 & 80.83 & 87.44 & 96.62 & 79.20 \\
    ODIN  & 37.33 & 48.27 & 69.80 & 48.91 & 80.83 & 87.44 & 96.62 & 79.20 \\
    \md   & 37.33 & 48.27 & 69.80 & 48.91 & 80.83 & 87.44 & 96.62 & 79.20 \\
    \midrule
    GNNSafe & 17.66 & 30.13 & 50.20 & 27.42 & 56.69 & 79.14 & 96.58 & 64.40 \\
    GraphDE & 46.00 & 37.86 & 69.80 & 40.68 & 77.68 & 88.90 & 96.20 & 77.00 \\
    GOOD-D & /     & /     & /     & /     & /     & /     & /     & / \\
    \midrule
    OCGIN & /     & /     & /     & /     & /     & /     & /     & / \\
    OCGTL & /     & /     & /     & /     & /     & /     & /     & / \\
    GLocalKD & /     & /     & /     & /     & /     & /     & /     & / \\
    \midrule
    SGOOD & \textbf{48.66} & \textbf{48.66} & \textbf{71.60} & \textbf{51.82} & 80.33 & \textbf{89.14} & \textbf{96.66} & \textbf{79.40} \\
    \bottomrule
    \end{tabular}%
    }
  \label{tab:acc}%
\end{table}%

% \begin{table}[!th]
%   \centering
%   \caption{Performance with different
% backbones by AUROC (\%).  \textbf{Bold}: best. \underline{Underline}: runner-up.}
%   \resizebox{0.8\textwidth}{!}{
%     \begin{tabular}{cccccccc}
%     \toprule
%     Backbone & Method & ENZYMES & IMDB-M & IMDB-B & BACE  & BBBP  & DrugOOD \\
%     \midrule
%     \multirow{5}[2]{*}{GCN} & \md & {\underline{70.04}}  & \underline{71.27}  & 53.46  & \underline{72.68}  & 54.97  & \underline{66.01}  \\
%           & GraphDE & 61.40  & 68.44  & 29.13  & 53.24  & 52.50  & 56.61  \\
%           & GOOD-D & 41.96  & 61.71  & 59.53  & 72.52  & \underline{58.91}  & 61.79  \\
%           & OCGIN & 64.35  & 57.46  & \underline{64.08}  & 67.54  & 51.23  & 59.30  \\
%           & SGOOD & \textbf{71.26 } & \textbf{73.52 } & \textbf{65.91 } & \textbf{83.42 } & \textbf{62.76 } & \textbf{72.52 } \\
%     \midrule
%     \multirow{5}[2]{*}{GraphSage} & \md & 68.07  & 48.06  & 43.63  & \underline{73.60}  & 53.88  & \underline{64.55}  \\
%           & GraphDE & 61.37  & \textbf{69.65 } & 28.28  & 53.24  & 52.50  & 56.66  \\
%           & GOOD-D & 45.55  & 57.02  & 23.90  & 73.15  & \underline{56.85}  & 61.57  \\
%           & OCGIN & \textbf{71.75 } & 36.86  & \textbf{71.44 } & 57.47  & 46.65  & 63.82  \\
%           & SGOOD & \underline{70.21}  & \underline{68.63}  & \underline{61.59}  & \textbf{82.22 } & \textbf{59.50 } & \textbf{68.60 } \\
%     \bottomrule
%     \end{tabular}%
%     }
%   \label{tab:backbone}%
% \end{table}%

\paragraph{Performance under different backbones other than GIN.}
We evaluate the performance of \algo and competitors when changing the GIN backbone to GCN~\citep{kipf2017semi} and GraphSage~\citep{hamilton2017inductive}. Table~\ref{tab:backbone} reports the results.
Observe that, with GCN backbone, compared with the baselines, \algo consistently achieves the best scores; with GraphSage backbone, \algo is the best on BACE, BBP, DrugOOD, and the second best on other datasets. The results validate the versatility/robustness of \algo to differnt backbones.

% Table generated by Excel2LaTeX from sheet 'Sheet4'

\begin{figure}[!t] 
% \vspace{-1em}
    \centering 
    \includegraphics[width=1\linewidth]{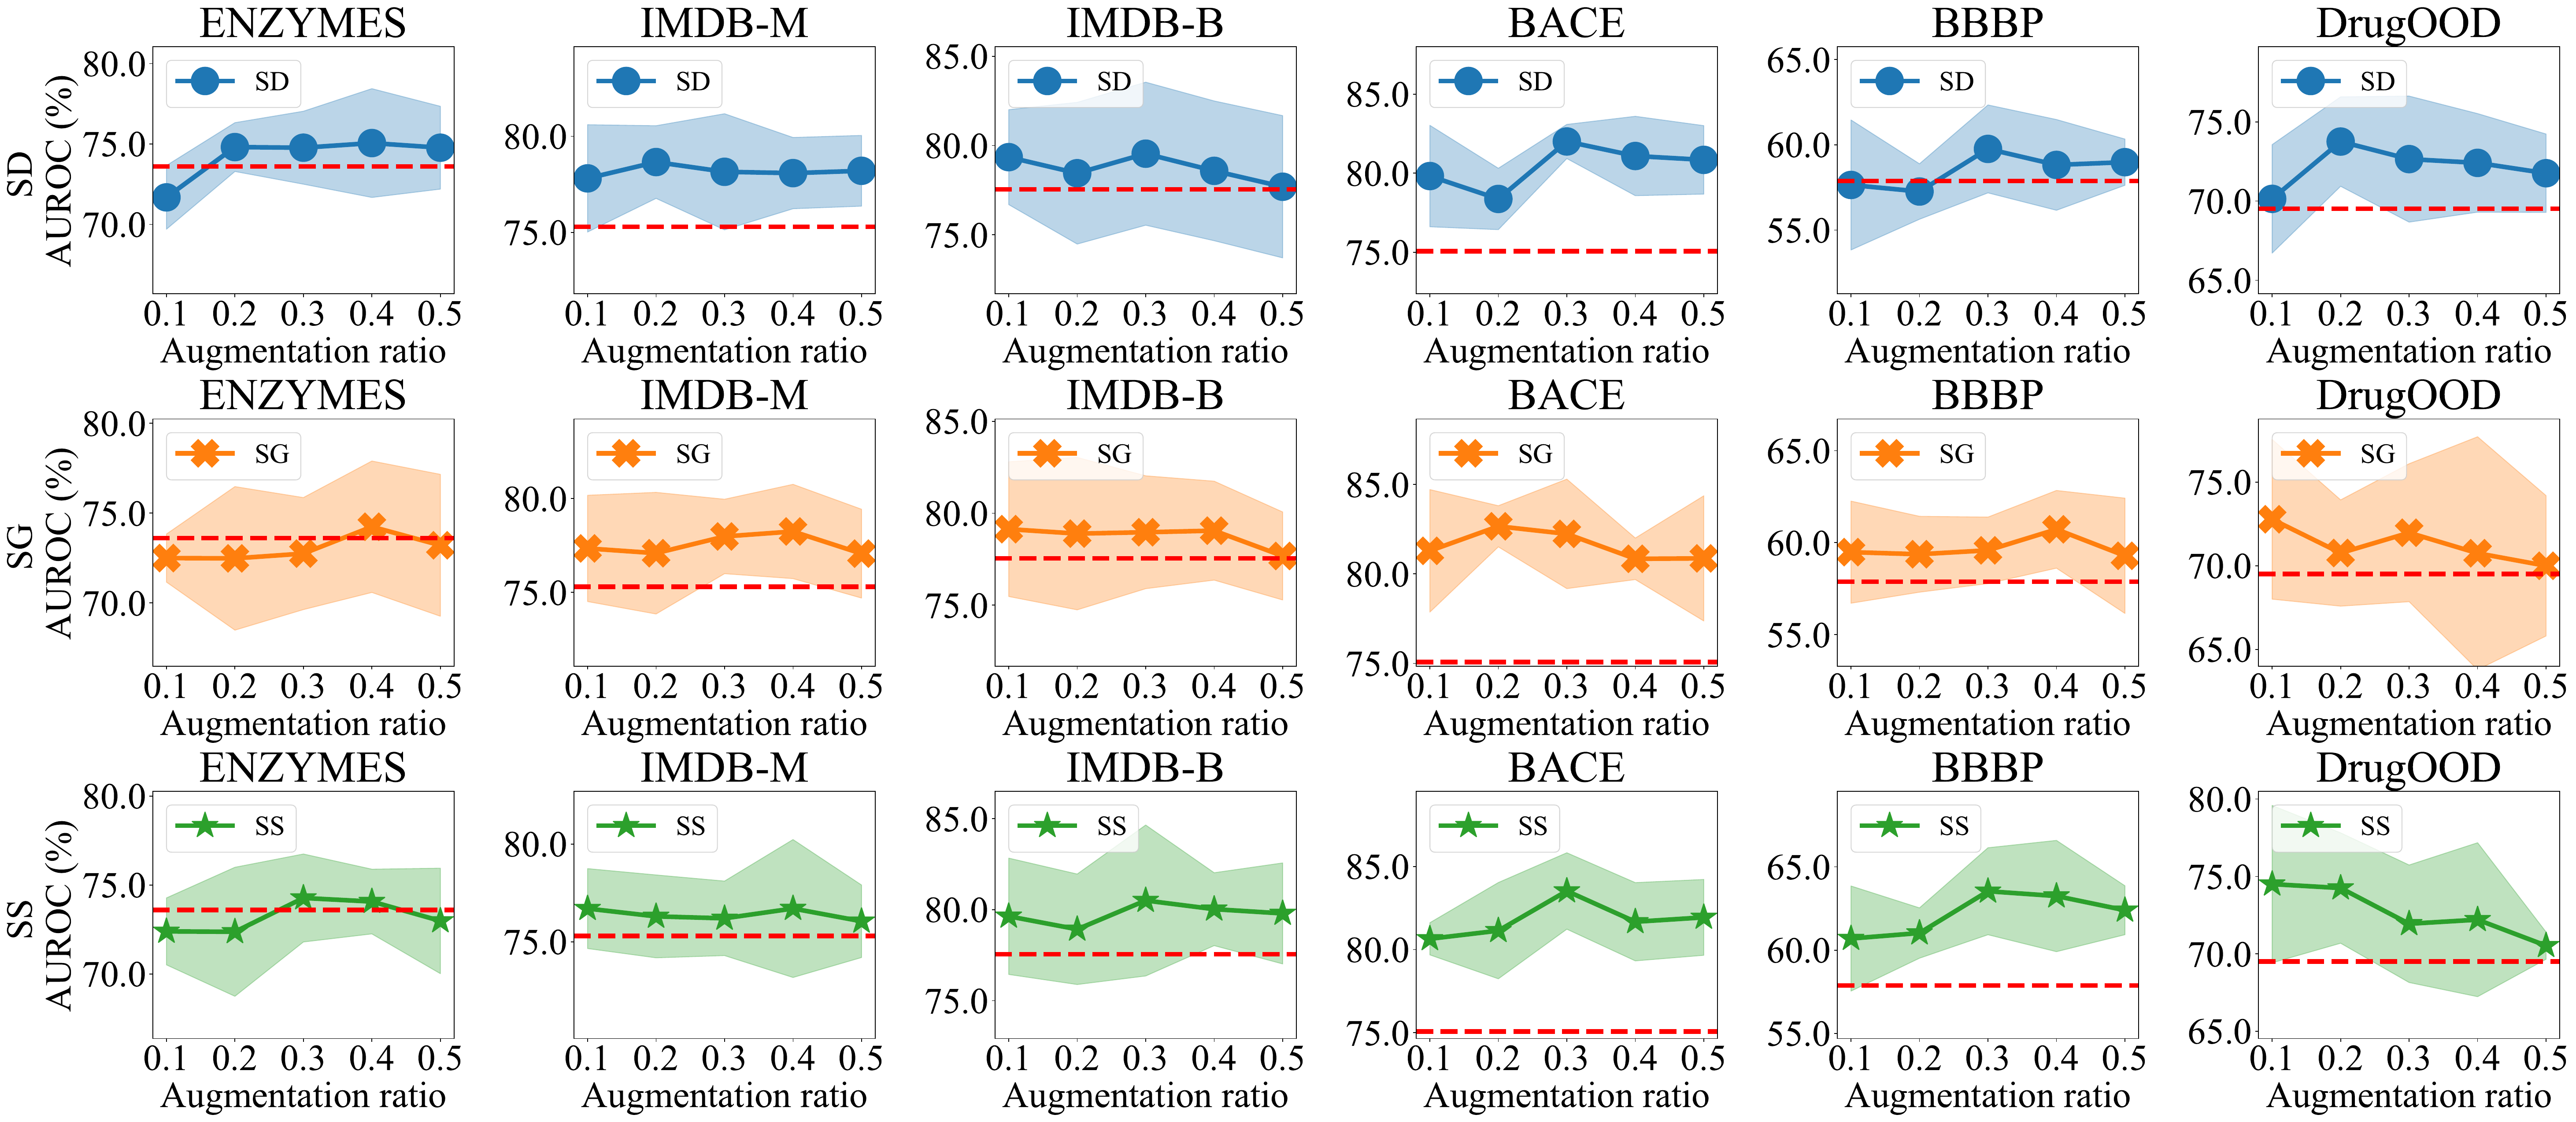}
    % \vspace{-1em}
    \caption{OOD detection performance of \algo when augmentation ratio varies by \auc (\%) on all the three substructure-preserving graph augmentations, SD, SG, and SS. The dotted red line indicates the performance of $\text{\algo}\backslash\text{CL}$ without any augmentation, which serves as a base performance. The area in color represents standard deviation.}
    \vspace{-1pt}
    \label{fig:ratio} 
\end{figure}

\paragraph{The effect of augmentation ratio.} We conduct experiments to study the effect of augmentation ratio on the three substructure-preserving  graph augmentations (SD, SG, SS) introduced in Section~\ref{sec::augmentations}. Specially,  
we fix $\mathcal{T}_{0}$ as $I$ that indicates no augmentation, set $\mathcal{T}_{1}$ as one of the three augmentations, and vary the augmentation ratio (dropping ratio/substitution ratio) from $0.1$ to $0.5$. Intuitively, larger augmentation ratio leads to harder contrastive tasks.  Figure \ref{fig:ratio} reports the results, and the dotted red line indicates the performance of $\text{\algo}\backslash\text{CL}$ without any augmentation  for calibration.
First, for all three substructure-preserving graph augmentations, under most augmentation ratio settings, we can achieve better performance than the red-dot baseline. 
Second, the three augmentations usually achieve the most significant performance improvement in \algo under moderate augmentation ratio (\eg 0.3 and 0.4).

% Overall, the three augmentations will lead to the most significant performance improvement on \algo  under moderate augmentation ratio (0.3 and 0.4). We also observe that too simple tasks, where augmentation ratio is low, will lead to performance drop. For example,all the three augmentations achieves performance inferior to $\text{\algo}\backslash\text{CL}$ when augmentation ratio is 0.1 on \enzymes. 

\begin{figure}[!t] 
% \vspace{-1em}
    \centering 
    \includegraphics[width=1\linewidth]{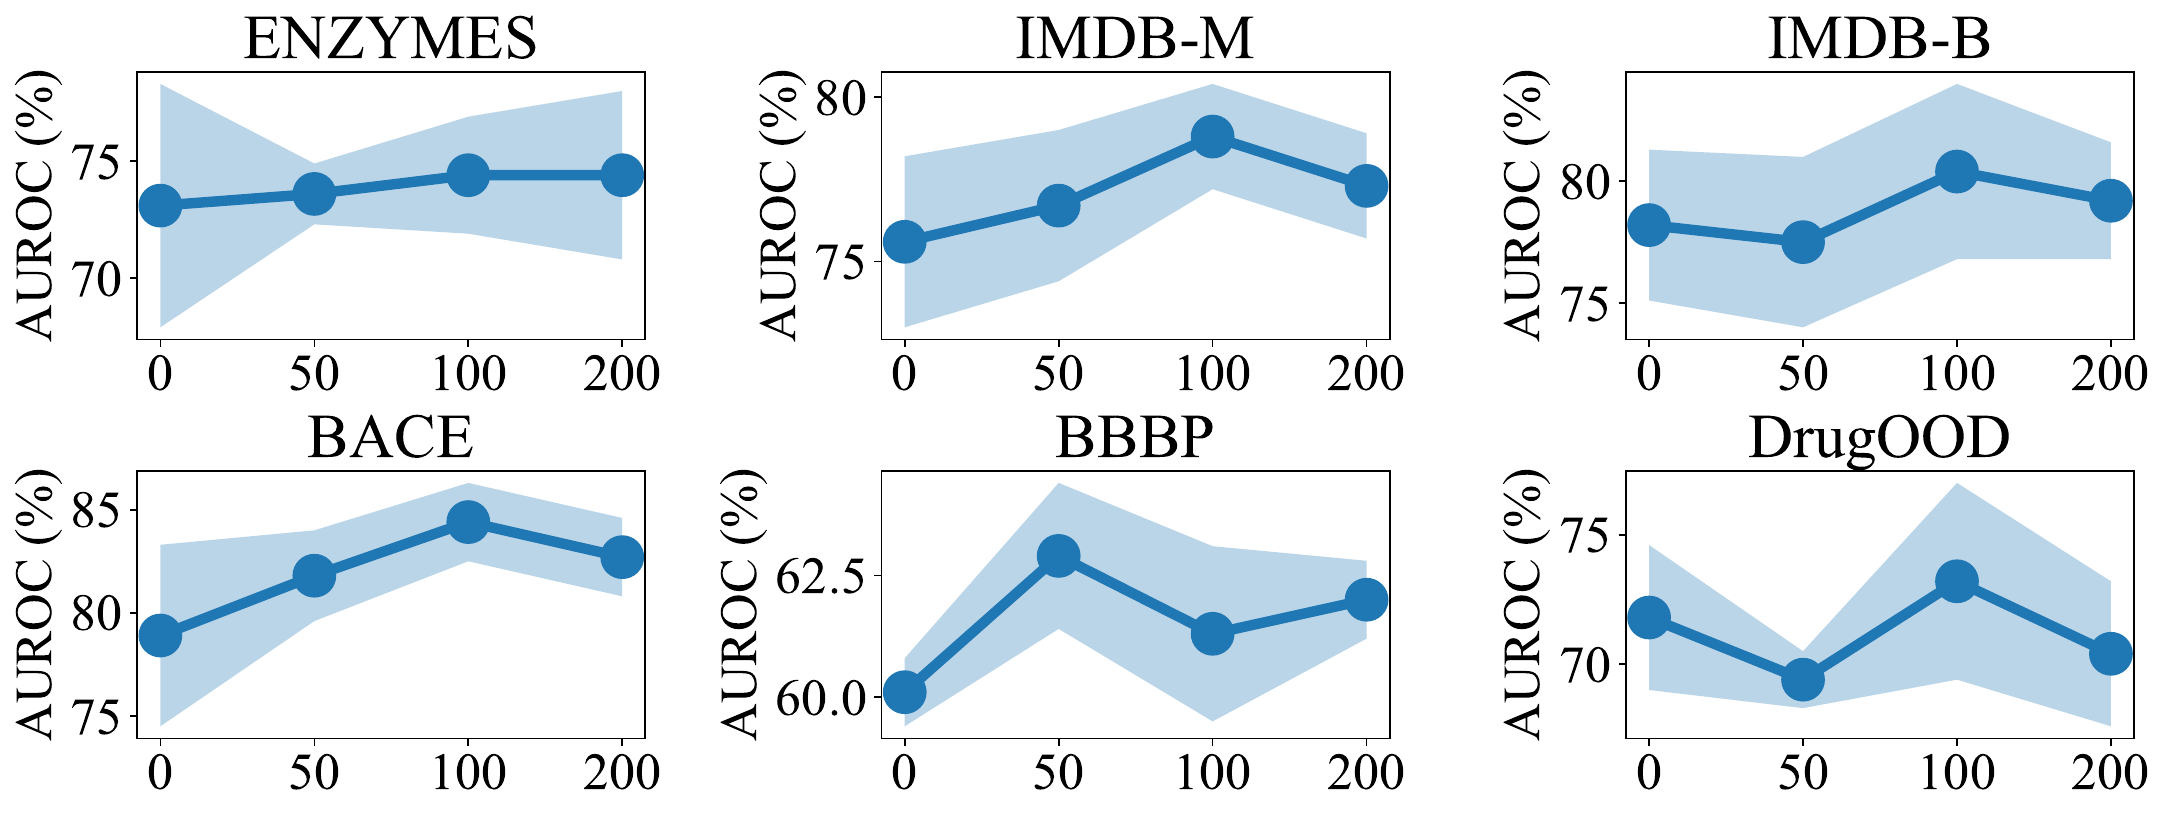}
    % \vspace{-1em}
    \caption{OOD detection performance  of \algo by \auc (\%) when the number of pretraining epochs $T_{PT}$ varies from 0 to 200, with colored area representing standard deviation.}
    \label{fig:epochs} 
\end{figure}

\paragraph{The effect of pretraining epochs.}
 We conduct experiments to study the effect of pretraining epochs $T_{PT}$ from 0 to 200. As shown in Figure~\ref{fig:epochs}, compared to \algo without first-stage pretraining ($T_{PT}=0$), pretraining  improves \algo's performance. We also found that excessive pretraining can sometimes have negative effects. For example, when $T_{PT}=200$, \algo's performance decrease  on all datasets except \enzymes. We speculate the reason is that excessive pretraining makes task-agnostic information dominate, with a negative impact on the \algo's ability to learn from class labels. As $T_{PT}=100$ generally leads to competitive performance across all datasets, 
 we set the default value of  $T_{PT}$ to 100.
\begin{figure}[!t] 
% \vspace{-1em}
    \centering 
    \includegraphics[width=1\linewidth]{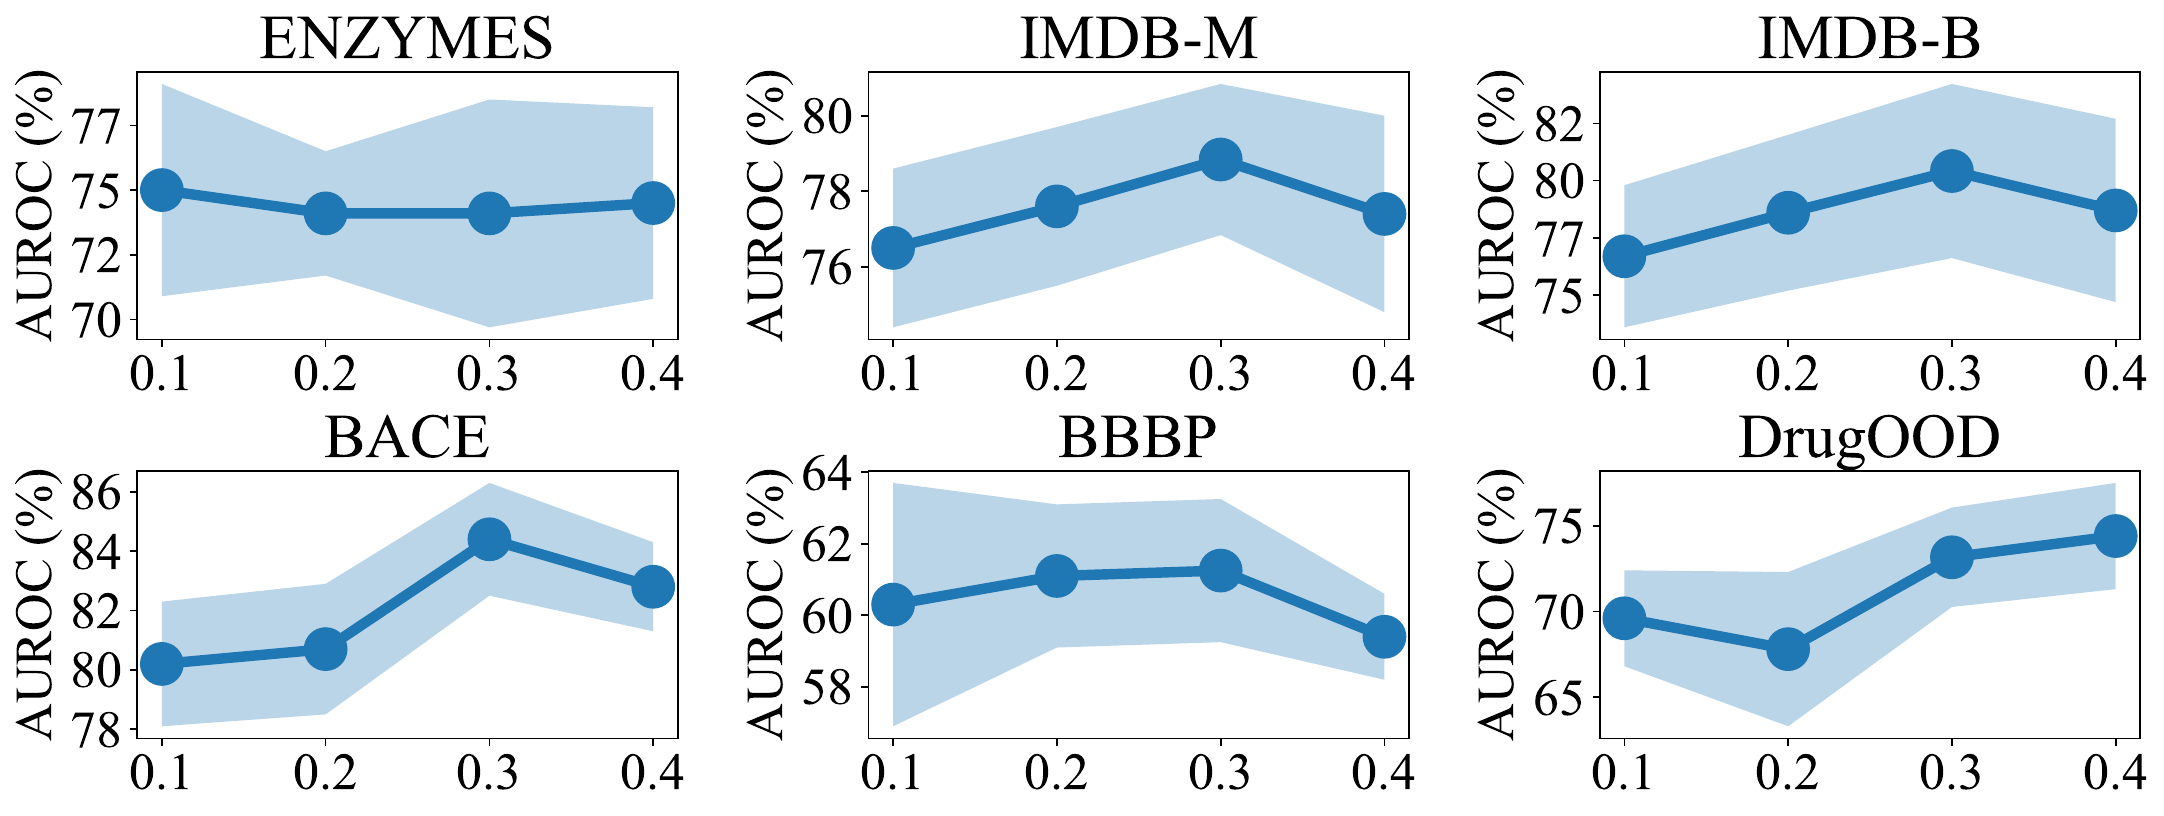}
    % \vspace{-1em}
    \caption{OOD detection results  of \algo  by \auc (\%) when the weight of the contrastive loss $\alpha$ varies from 0 to 1, with colored area representing standard deviation.}
    \label{fig:weight} 
\end{figure}

\paragraph{The effect of $\alpha$.}

 We vary  the weight of the contrastive loss $\alpha$ from 0 to 1 to study the effect. As shown in Figure~\ref{fig:weight}, compared to \algo fine-tuned solely by $\mathcal{L}_{CE}$ (\ie $\alpha=0$), fine-tuning \algo with both $\mathcal{L}_{CE}$ and $\mathcal{L}_{CL}$ generally leads to better performance. 
 %The reason is that moderate $\mathcal{L}_{CL}$ in fine-tuning helps \algo keep high-level, task-agnostic knowledge.  
 As $\alpha = 0.1$ usually leads to competitive performance across all datasets, we set the default value of  $\alpha$ to 0.1 in \algo.

\paragraph{The effect of the number of negative samples in $\mathcal{L}_{CL}$. } We conduct experiments to study the effect of the number of  negative samples used in  contrastive loss $\mathcal{L}_{CL}$ (Eq.\eqref{eq:lossCL}). Following the established convention in graph contrastive learning~\cite{you2020graph}, pairs of augmented graphs originating from the same graph are treated as positive pairs, while pairs generated from different graphs within the batch are considered negative pairs. In such a way, in a $B$-size batch, for every $G_i$, it will have $2B-2$ negative samples, as shown in the denominator of Eq.\eqref{eq:lossCL}. Apparently the number of negative samples is related to batch size $B$. We vary $B$ from 16 to 256 to evaluate sensitivity of SGOOD w.r.t. the number of negative samples, and report the results in  Figure~\ref{fig:batch} . Observe that as increasing from 16 to 128, the overall performance increases and then becomes relatively stable, which proves the effectiveness of the augmentation techniques developed in \algo and also validates the superior performance of \algo when varying  batch size and the number of negative samples.

%For example, \jieming{blabla}.

\textbf{Visualizing pairwise combinations of all augmentations.}
In Figure \ref{fig:heatmap}, we exhaust the pairwise combinations of all options in $\mathcal{A}=\{\text{\underline{I, SD, SG, SS}}\}$ and visualize the \auc gain on graph-level OOD detection over $\text{\algo}\backslash\text{A}$ without graph augmentations. As shown in Figure \ref{fig:heatmap}, most combinations achieve positive gains for effective OOD detection.

\begin{figure}[!t] 
% \vspace{-1em}
    \centering 
    \includegraphics[width=1\linewidth]{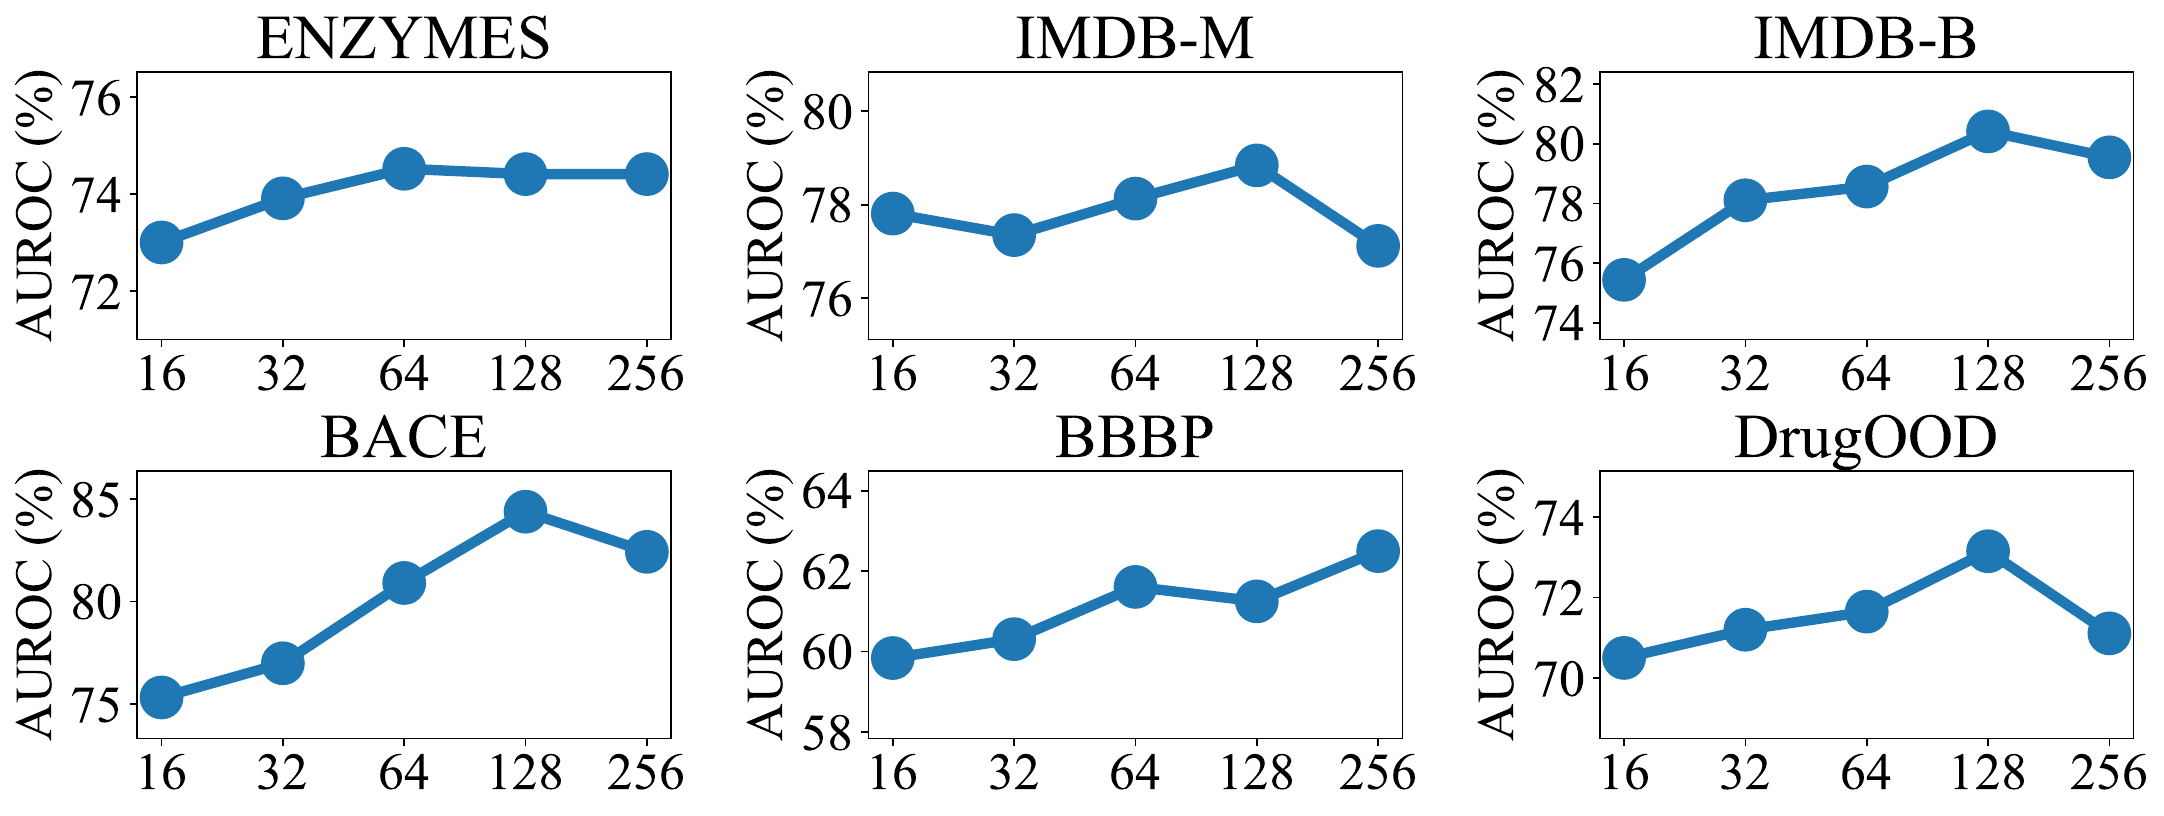}
    % \vspace{-1em}
    \caption{ OOD detection results  of \algo  by \auc (\%) when the batch size $B$ varies from 16 to 256.}
    \label{fig:batch} 
\end{figure}

\begin{figure}[!t] 
% \vspace{-1em}
    \centering 
    \includegraphics[width=0.9\linewidth]{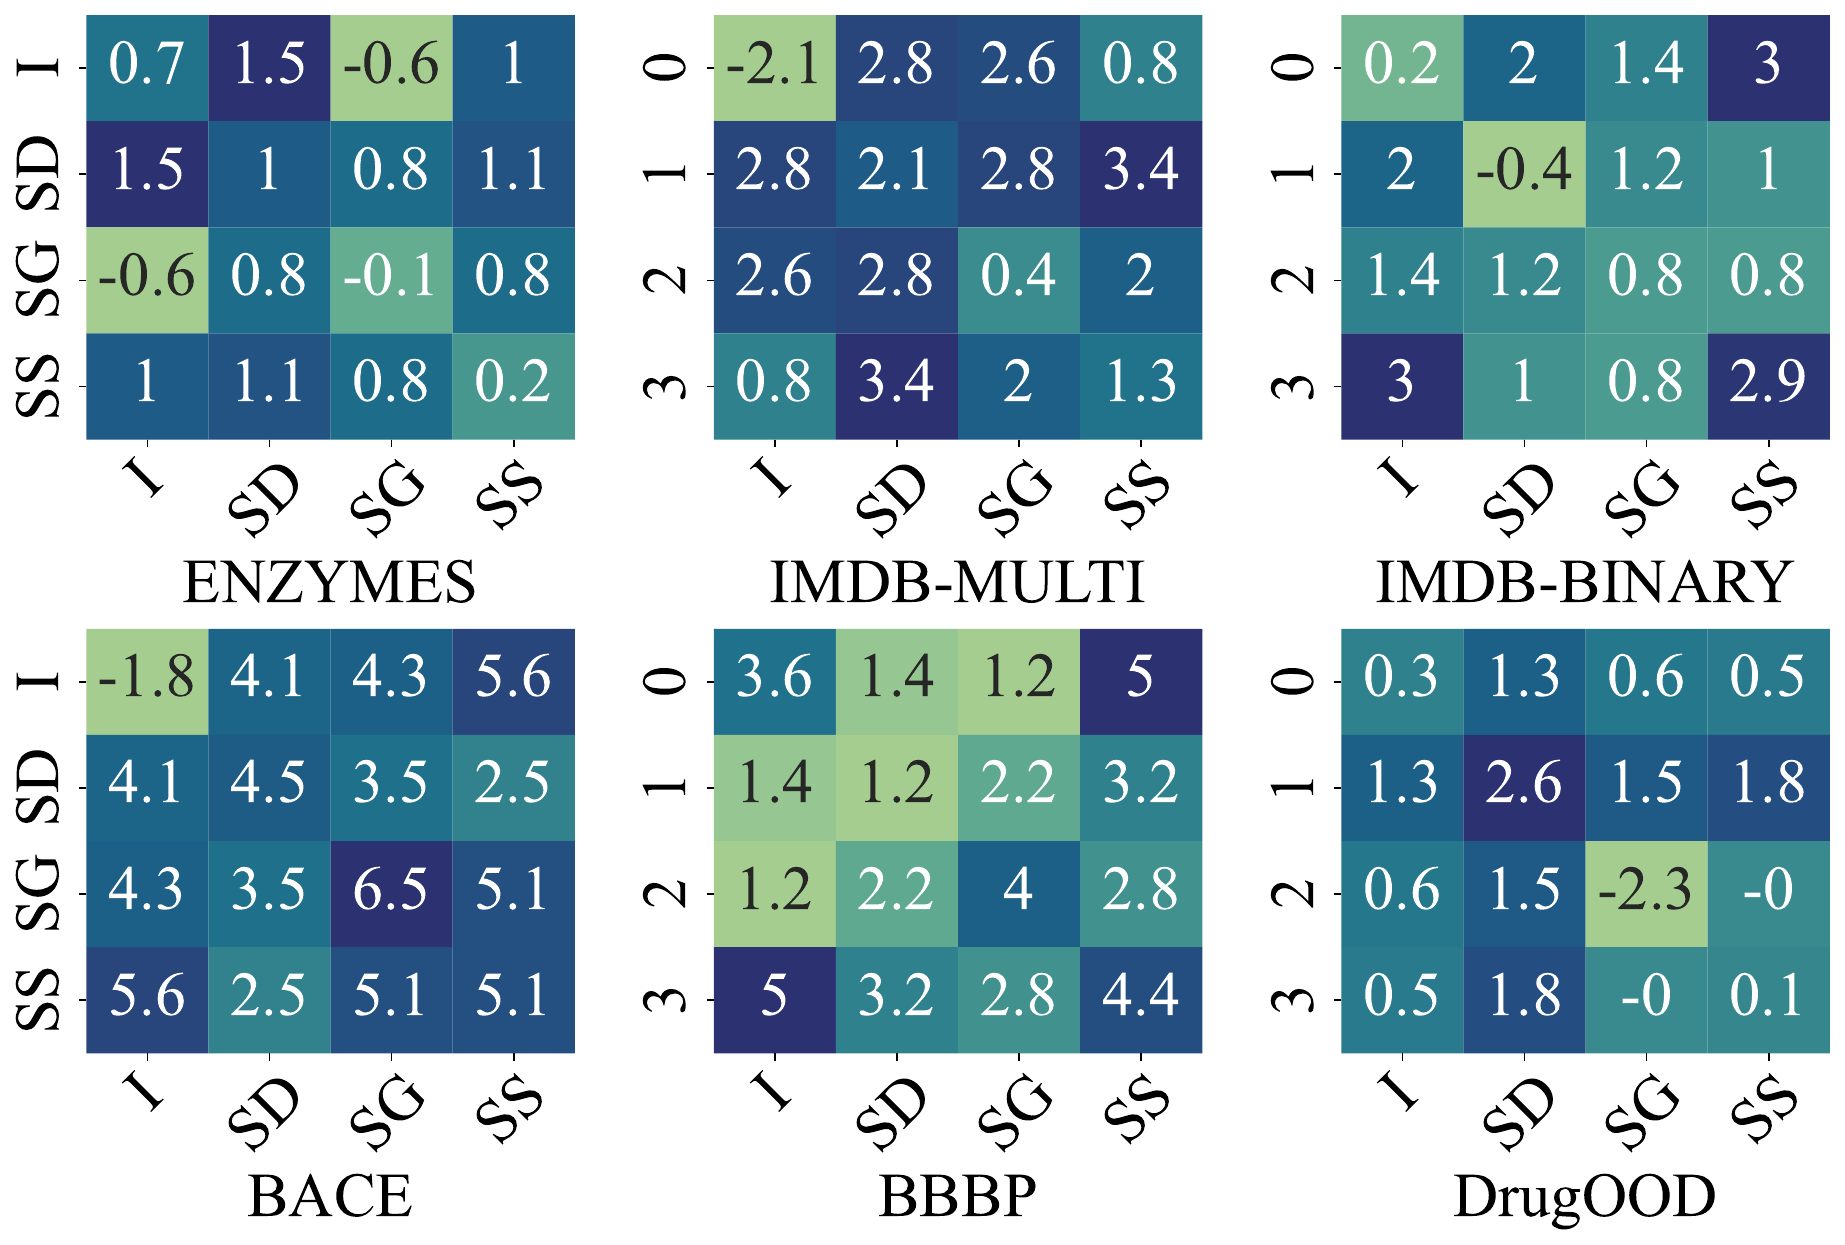}
    % \vspace{-1em}
      \vspace{-2mm}
    \caption{\auc gain (\%) of \algo  compared with $\text{\algo}\backslash\text{A}$ without graph augmentations.}
    \vspace{-3mm}
    \label{fig:heatmap} 
\end{figure}

\begin{table}[!t]
  \centering
  \caption{Comparison of training time per epoch and inference time per epoch of all the methods on six datasets by seconds (s).}
  \resizebox{1.0\textwidth}{!}{
    \begin{tabular}{ccccccccccccccccc}
    \toprule
    \multirow{2}[3]{*}{Method} & \multicolumn{2}{c}{ENZYMES} & \multicolumn{2}{c}{IMDB-B} & \multicolumn{2}{c}{IMDB-M} & \multicolumn{2}{c}{\reddit} & \multicolumn{2}{c}{BACE} & \multicolumn{2}{c}{BBBP} & \multicolumn{2}{c}{\hiv} & \multicolumn{2}{c}{DrugOOD} \\
\cmidrule{2-17}          & Train (s) & Test (s) & Train (s) & Test (s) & Train (s) & Test (s) & Train (s) & Test (s) & Train (s) & Test (s) & Train (s) & Test (s) & Train (s) & Test (s) & Train (s) & Test (s) \\
    \msp  & 0.119  & 0.008  & 0.090  & 0.007  & 0.077  & 0.007  & 0.890  & 0.260  & 0.053  & 0.005  & 0.055  & 0.006  & 2.740  & 0.200  & 0.078  & 0.005  \\
    \energy & 0.119  & 0.008  & 0.090  & 0.007  & 0.077  & 0.007  & 0.890  & 0.260  & 0.053  & 0.005  & 0.055  & 0.006  & 2.740  & 0.200  & 0.078  & 0.005  \\
    \odin & 0.119  & 0.026  & 0.090  & 0.022  & 0.077  & 0.021  & 0.890  & 0.420  & 0.053  & 0.016  & 0.055  & 0.013  & 2.740  & 0.300  & 0.078  & 0.020  \\
    \md   & 0.119  & 0.020  & 0.090  & 0.019  & 0.077  & 0.018  & 0.890  & 0.400  & 0.053  & 0.016  & 0.055  & 0.019  & 2.740  & 0.300  & 0.078  & 0.019  \\
    \midrule
    \graphde & 1.692  & 0.358  & 1.392  & 0.292  & 1.175  & 0.380  & 176.400  & 0.120  & 0.950  & 0.155  & 0.696  & 0.138  & 43.770  & 9.620  & 1.020  & 0.232  \\
    \good & 0.257  & 0.006  & 0.197  & 0.008  & 0.171  & 0.009  & 17.550  & 0.710  & 0.157  & 0.006  & 0.095  & 0.008  & 5.160  & 0.010  & 0.230  & 0.006  \\
    \midrule
    \ocgin & 0.123  & 0.005  & 0.086  & 0.006  & 0.079  & 0.005  & 1.650  & 0.170  & 0.075  & 0.005  & 0.044  & 0.005  & 2.900  & 0.050  & 0.099  & 0.005  \\
    \glkd & 0.072  & 0.853  & 0.054  & 0.629  & 0.203  & 0.707  & 142.000  & 37.670  & 0.052  & 0.527  & 0.035  & 0.320  & 4.220  & 30.420  & 0.067  & 0.788  \\
    \midrule
    \algo & 0.161  & 0.030  & 0.137  & 0.027  & 0.138  & 0.028  & 0.980  & 0.130  & 0.085  & 0.025  & 0.058  & 0.028  & 3.970  & 0.300  & 0.124  & 0.030  \\
     \bottomrule
    \end{tabular}%
    }
  \label{tab:time}
\end{table}%

\paragraph{Model efficiency.}
We compare the training time per epoch and inference time per epoch in seconds of all methods, with results in Table~\ref{tab:time}. 
%As the training of \algo involves two stages, we report the average time cost of fine-tuning stage which is higher than pretraining. 
Compared with other graph-level OOD detection competitors, including \graphde and \good, \algo requires less time to train. 
Compared with all methods, including the methods originally designed for image data, \algo requires moderate time for training.
In terms of inference time, \algo is much more efficient than \graphde.  Although \good is more efficient in inference, it is not as accurate as \algo in OOD detection as shown in Table \ref{tab:overall}.
Considering together the time cost 
in Table \ref{tab:time} and the effectiveness in Table \ref{tab:overall}, we can conclude
that \algo has superior accuracy for graph-level OOD detection,
while being reasonably efficient.

% \begin{table}[htbp]
% % \vspace{-\baselineskip}  
% \centering
%   \caption{Varying $L_{1}$ and $L_{2}$ in \algo (\auc).}
%     \vspace{-1mm}
%     \setlength{\tabcolsep}{2pt}

%   \resizebox{0.45\textwidth}{!}{
%     \begin{tabular}{ccccccccc}
%     \toprule
%     $L_{1}$ & $L_{2}$ & \enzymes & \multi & \binary & \bbbp  & \bace  & \drug \\
%     \midrule
%     4     & 1     & 74.00  & 77.13  & \textbf{81.00 } & 80.43  & 62.00  & 71.17  \\
%     3     & 2     & \textbf{74.41 } & \textbf{78.84 } & 80.42  & \textbf{84.40 } & 61.25  & \textbf{73.16 } \\
%     2     & 3     & 73.63  & 76.03  & 79.05  & 80.34  & \textbf{62.26 } & 69.12  \\
%     1     & 4     & 74.22  & 77.83  & 76.79  & 76.62  & 61.08  & 68.01  \\
%     \bottomrule
%     \end{tabular}%
%   \label{tab:layers}%
%   }
% \vspace{-2pt}
% \end{table}

\begin{figure}[!t] 
% \vspace{-1em}
    \centering 
    \includegraphics[width=0.8\linewidth]{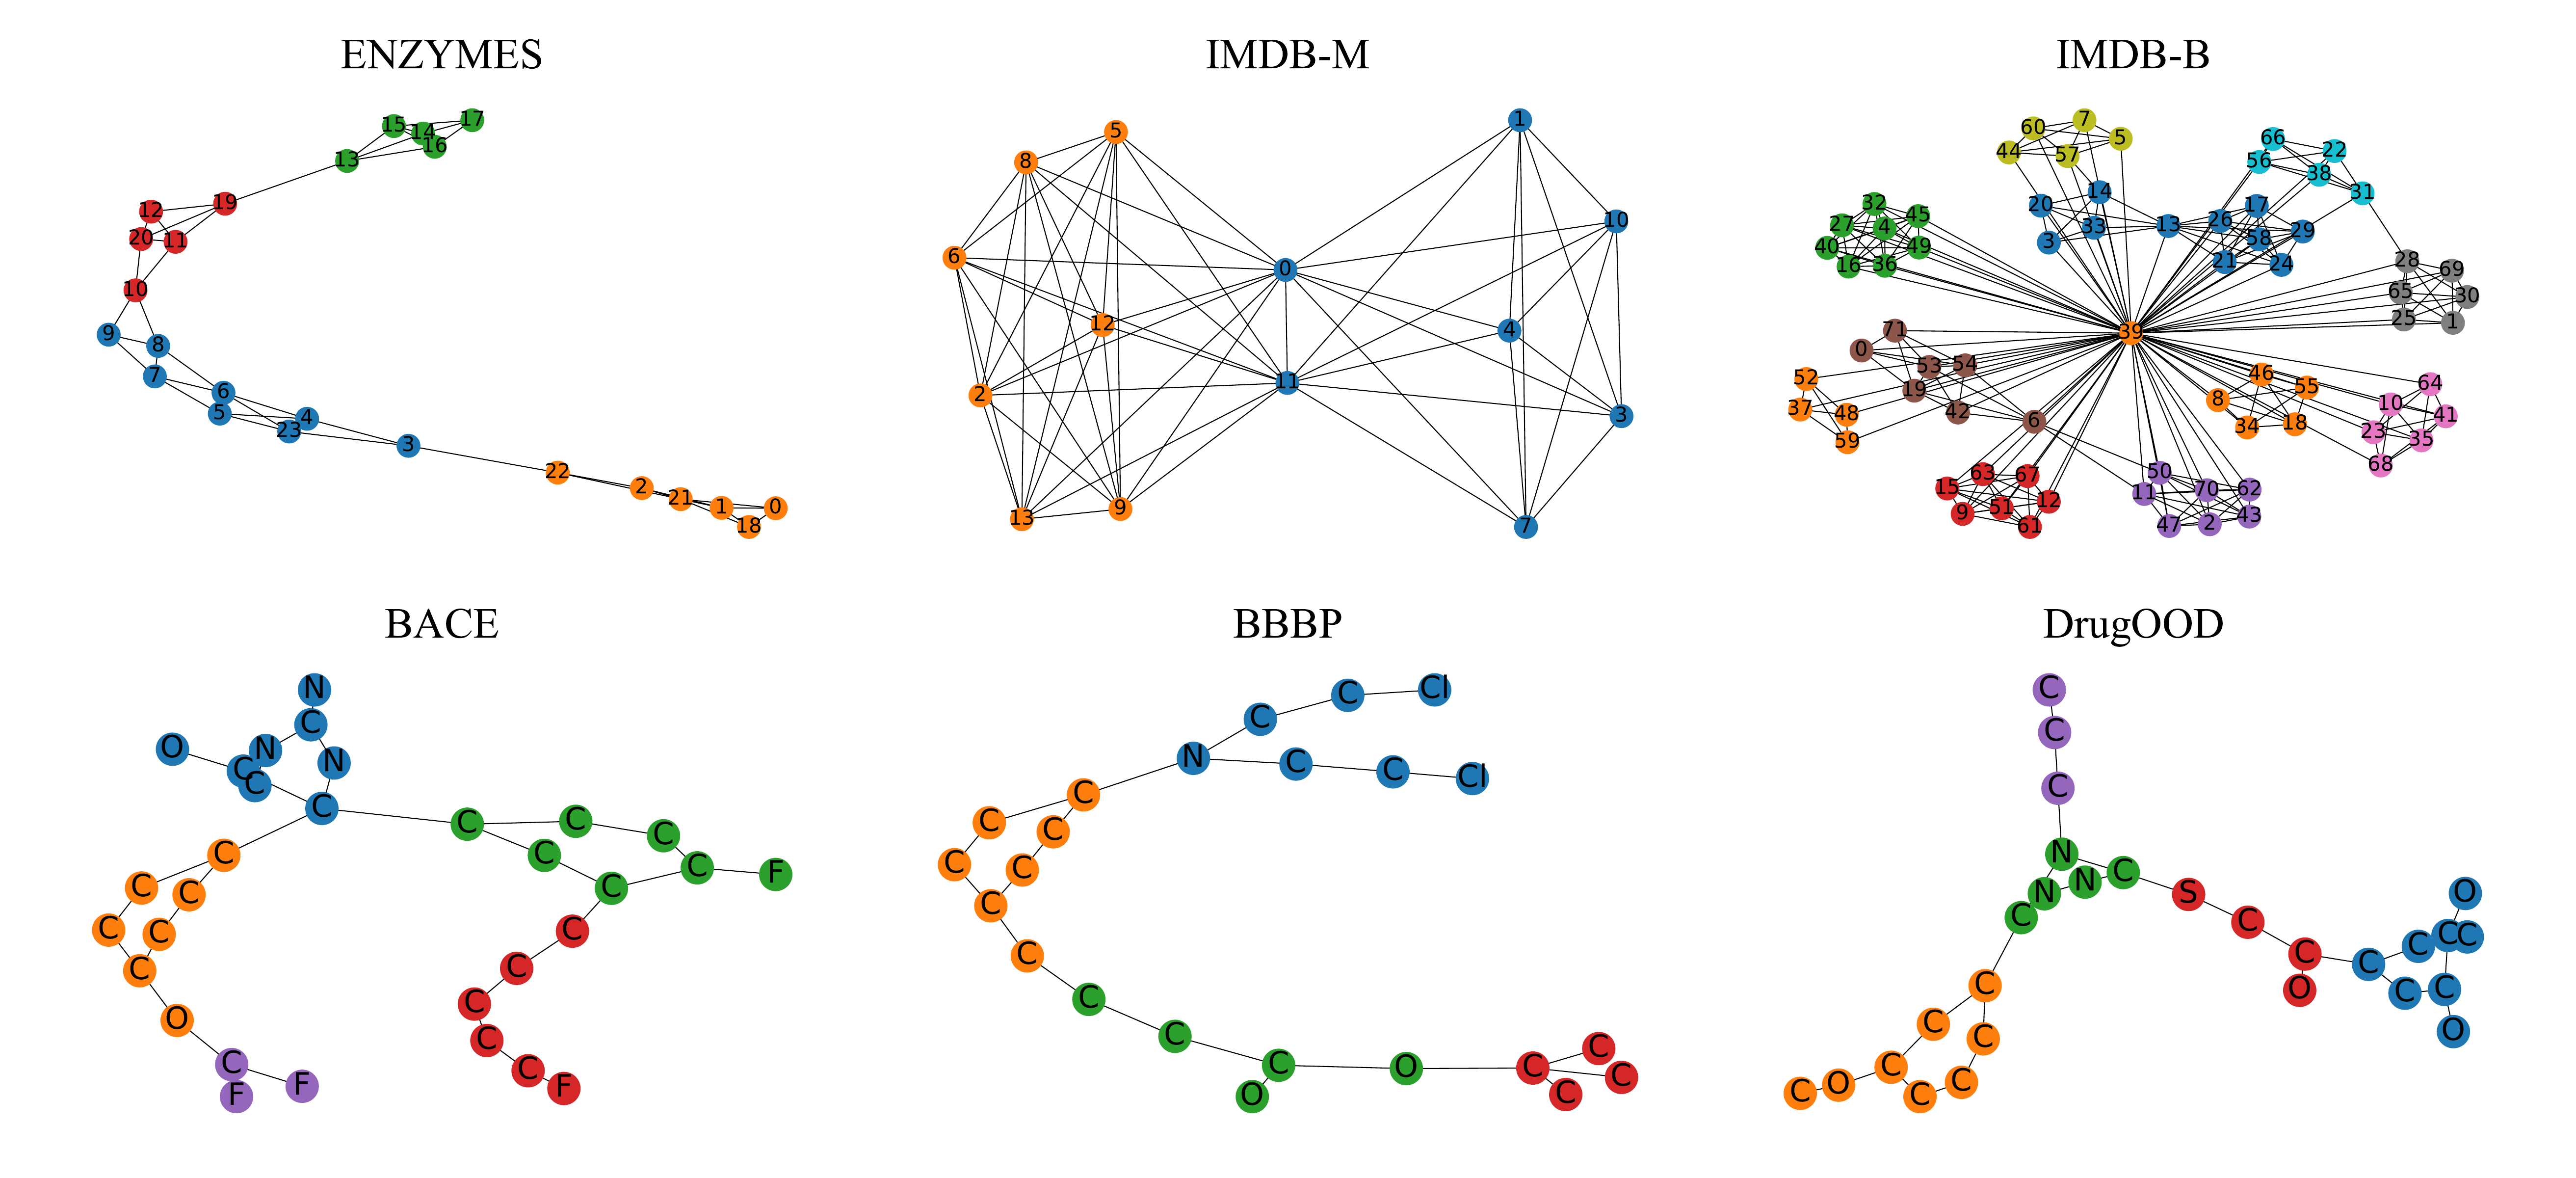}
    % \vspace{-1em}
    \caption{Different colors indicate different substructures. For molecular graphs, we label the nodes with atom types. For graphs of other types, we label the nodes with node IDs.}
    \vspace{-1em}
    \label{fig:visualization} 
\end{figure}

% \paragraph{Varying $L_1$ and $L2$.} 
% In the above experiments, we fix the layers of the two GINs in the two-level graph encoding in Section \ref{sec::substructure} to be $L_1=3$ and $L_2=2$ as default. If we search $L_1$ and $L_2$, it is possible to get even better OOD detection results, as shown  in Table \ref{tab:layers} where $L_1$ and $L_2$ are varied with their sum fixed to be 5. For example, on BACE with $L_1$=$2$ and $L_2$=$3$, \auc is 62.26\%, about 1\% higher than the default setting.

\paragraph{Substructure Visualization.}
In \algo, we adopt the modularity-based community detection method~\citep{clauset2004finding} to detect substructures in a graph. We demonstrate the detected substructures in different datasets in Figure~\ref{fig:visualization}. We observe that dense cliques in protein networks (\enzymes) and social networks (\multi, \binary) are separated as substructures in \algo. For molecular graphs, the rings that play a critical role in the properties of molecules\citep{zhumathcal} are detected in \algo. As the cliques and rings can not be captured by graph representations generated by GNNs based on message passing and flat pooling~\citep{chen2020can} while \algo can generate substructure-enhanced graph representations, it explains why \algo achieves superior performance in graph-level OOD detection.

% Table generated by Excel2LaTeX from sheet 'layer'

\section{Pseudo-code of \algo}\label{apx:algo}
\vspace{-2mm}

We present the pseudo code of \algo for training and testing in Algorithm \ref{algo:train} and \ref{algo:test} respectively.
\vspace{-4mm}

\begin{algorithm}[!h]
\small	
\caption{Pseudo-code of \algo (Training)}\label{algo:train}
	\DontPrintSemicolon
	\SetNoFillComment
 \textbf{Input:} Training dataset $\Din_{tr}=\{(G_i,y_i)\}^n_{i=1}$,  testing set $\Dtest$, weight of the contrastive loss $\alpha$, number of first-stage pretraining epoch $T_{PT}$, number of second-stage fine-tuning epoch $T_{FT}$\\
 \tcp{Super graph construction}
 Construct   super graphs of substructures $\{\mathcal{G}_{i}\}_{i=1}^{n}$ of all $G_{i} \in \Din_{tr}$;\\
 \tcp{First  stage}
 \For {$epoch=1,2,\ldots, T_{PT}$}{Randomly split training graphs $\Din_{tr}$ into batches $\mathcal{B}$ with batch size $B$;\\
    \For {$\{G_{i}\}_{i=1}^{B} \in \mathcal{B}$}{
        \For {$G_{i} \in \{G_{i}\}_{i=1}^{B}$}{
    Obtain augmented super graphs $\widehat{\mathcal{G}}_{i,0}, \widehat{\mathcal{G}}_{i,1}$ by applying  $\mathcal{T}_{0}$ and $\mathcal{T}_{1}$ to $\mathcal{G}_{i}$;\\
    Obtain augmented graphs $\widehat{G}_{i,0}, \widehat{G}_{i,1}$ according to  $\widehat{\mathcal{G}}_{i,0}, \widehat{\mathcal{G}}_{i,1}$;\\
    Calculate $\mathbf{h}_{\widehat{\mathcal{G}}_{i,0}}$ and $\mathbf{h}_{\widehat{\mathcal{G}}_{i,1}}$ using $(\widehat{G}_{i,0}, \widehat{\mathcal{G}}_{i,0})$ and $(\widehat{G}_{i,1}, \widehat{\mathcal{G}}_{i,1})$ by  Eq.\eqref{eq:node_mp}-\eqref{eq:sub_pool};\\
    Obtain $\mathbf{u}_{\widehat{\mathcal{G}}_{i,0}} = \frac{\psi(\mathbf{h}_{\widehat{\mathcal{G}}_{i,0}})}{||\psi(\mathbf{h}_{\widehat{\mathcal{G}}_{i,0}})||}$ and $\mathbf{u}_{\widehat{\mathcal{G}}_{i,1}} = \frac{\psi(\mathbf{h}_{\widehat{\mathcal{G}}_{i,1}})}{||\psi(\mathbf{h}_{\widehat{\mathcal{G}}_{i,1}})||}$ using shared projection head $\psi$ followed by $l_{2}$-normalization;\\}
    Calculate contrastive loss $\mathcal{L}_{CL}$ by Eq.\eqref{eq:lossCL};\\
    Update parameters using mini-batch gradient descent \wrt $\mathcal{L}_{CL}$;\\
    }}
 \tcp{Second stage}
 \For {$epoch=1,2,\ldots, T_{FT}$}{Randomly split training graphs $\Din_{tr}$ into batches $\mathcal{B}$ with batch size $B$;\\
    \For {$\{G_{i}\}_{i=1}^{B} \in \mathcal{B}$}{
        \For {$G_{i} \in \{G_{i}\}_{i=1}^{B}$}{
        Same as Lines 7-10 ;\\
        Calculate $\mathbf{h}_{\mathcal{G}_{i}}$ using $(G_{i}, \mathcal{G}_{i})$ by  Eq.\eqref{eq:node_mp}-\eqref{eq:sub_pool};\\
%    Obtain augmented super graphs $\widehat{\mathcal{G}}_{i,0}, \widehat{\mathcal{G}}_{i,1}$ by applying  $\mathcal{T}_{0}$ and $\mathcal{T}_{1}$ to $\mathcal{G}_{i}$;\\
 %   Obtain augmented graphs $\widehat{G}_{i,0}, \widehat{G}_{i,1}$ according to  $\widehat{\mathcal{G}}_{i,0}, \widehat{\mathcal{G}}_{i,1}$;\\
   % Calculate $\mathbf{h}_{\mathcal{G}_{i}}$, $\mathbf{h}_{\widehat{\mathcal{G}}_{i,0}}$, and $\mathbf{h}_{\widehat{\mathcal{G}}_{i,1}}$ using $(G_{i}, \mathcal{G}_{i})$, $(\widehat{G}_{i,0}, \widehat{\mathcal{G}}_{i,0})$, and $(\widehat{G}_{i,1}, \widehat{\mathcal{G}}_{i,1})$ by  Eq.\eqref{eq:node_mp}-\eqref{eq:sub_pool};\\
    
    %Obtain $\mathbf{u}_{\widehat{\mathcal{G}}_{i,0}} = \frac{\psi(\mathbf{h}_{\widehat{\mathcal{G}}_{i,0}})}{||\psi(\mathbf{h}_{\widehat{\mathcal{G}}_{i,0}})||}$ and $\mathbf{u}_{\widehat{\mathcal{G}}_{i,1}} = \frac{\psi(\mathbf{h}_{\widehat{\mathcal{G}}_{i,1}})}{||\psi(\mathbf{h}_{\widehat{\mathcal{G}}_{i,1}})||}$ using shared projection head $\psi$ followed by $l_{2}$-normalization;\\
    Calculate  prediction logits $\widehat{y}_{i}$ by applying linear transformation on $\mathbf{h}_{\mathcal{G}_{i}}$;\\
    }
    Calculate cross-entropy loss $\mathcal{L}_{CE}$ by Eq.\eqref{eq:lossce};\\    
    Calculate contrastive loss $\mathcal{L}_{CL}$ by Eq.\eqref{eq:lossCL};\\
    Update parameters using mini-batch gradient descent \wrt $\mathcal{L}_{CE}+\alpha \mathcal{L}_{CL}$;\\
    }}
 \tcp{Estimate class centroids and covariance matrix}
  \For {$G_{i} \in \Din_{tr}$}{
    Calculate $\{\mathbf{h}_{v}|v\in {V}_{i}\}$ and $\mathbf{h}_{\mathcal{G}_{i}}$ using $(G_{i}, \mathcal{G}_{i})$ by  Eq.\eqref{eq:node_mp}-\eqref{eq:sub_pool};\\
    Calculate $\mathbf{h}_{G_{i}}=\texttt{\small{READOUT}}(\{\mathbf{h}_{v}|v\in {V}_{i}\})$;\\
    Calculate $\mathbf{z}_{i} = \frac{\texttt{\small{CONCAT}}(\mathbf{h}_{G_{i}},\mathbf{h}_{\mathcal{G}_{i}})}{||\texttt{\small{CONCAT}}(\mathbf{h}_{G_{i}},\mathbf{h}_{\mathcal{G}_{i}})||_{2}}$;
  }
  Calculate estimated class centroids $\{\bm{\mu}_{c}\}_{c=1}^{C}$ 
and covariance matrix $\widehat{ \Sigma}$ by Eq.\eqref{eq:md};\\
\end{algorithm}

\begin{algorithm}[t]
\small	
\caption{Pseudo-code of \algo (OOD Detection During Testing)}\label{algo:test}
	\DontPrintSemicolon
	\SetNoFillComment
 \textbf{Input:} The trained \algo model $f$, testing set $\Dtest$, estimated class centroids $\{\bm{\mu}_{c}\}_{c=1}^{C}$ , estimated covariance matrix $\widehat{ \Sigma}$
 %, threshold of OOD score $\lambda$ 
 \\

 \tcp{Testing stage}
 \For{$G_{i}\in \Dtest$}{
 Construct super graph $\mathcal{G}_{i}$;\\
    Calculate $\{\mathbf{h}_{v}|v\in {V}_{i}\}$ and $\mathbf{h}_{\mathcal{G}_{i}}$ using $(G_{i}, \mathcal{G}_{i})$ and $f$ by  Eq.\eqref{eq:node_mp}-\eqref{eq:sub_pool};\\
     Calculate $\mathbf{h}_{G_{i}}=\texttt{\small{READOUT}}(\{\mathbf{h}_{v}|v\in {V}_{i}\})$;\\
    Calculate $\mathbf{z}_{i} = \frac{\texttt{\small{CONCAT}}(\mathbf{h}_{G_{i}},\mathbf{h}_{\mathcal{G}_{i}})}{||\texttt{\small{CONCAT}}(\mathbf{h}_{G_{i}},\mathbf{h}_{\mathcal{G}_{i}})||_{2}}$;\\
    Calculate OOD score $S(G_i)$ by Eq.\eqref{eq:md};\\
    \If{$G_i$ is not OOD based on $S(G_i)$}{
    Perform classification on $G_i$ via  prediction logits $\widehat{y}_{i}$ by applying linear transformation on $\mathbf{h}_{\mathcal{G}_{i}}$;
    }
 }
\end{algorithm}

\begin{table}[!h]
\centering
  \caption{ ID graph classification performance measured by  \acc.  All results are reported in percentage \% (mean ± std). {/ indicates that \acc is not applicable for  unsupervised  methods.} }
  \resizebox{0.48\textwidth}{!}{
  % \setlength{\tabcolsep}{1.2pt}
  % \hspace{-3mm}
    \begin{tabular}{ccccccccc}
    \toprule
    \multicolumn{1}{l}{Method} & \multicolumn{1}{l}{ENZYMES} & \multicolumn{1}{l}{IMDB-M} & \multicolumn{1}{l}{IMDB-B} & \multicolumn{1}{l}{\reddit} & \multicolumn{1}{l}{BACE} & \multicolumn{1}{l}{BBBP} & \multicolumn{1}{l}{HIV} & \multicolumn{1}{l}{DrugOOD} \\
    \midrule
    MSP   & 37.33 & 48.27 & 69.80 & 48.91 & 80.83 & 87.44 & 96.62 & 79.20 \\
    Energy & 37.33 & 48.27 & 69.80 & 48.91 & 80.83 & 87.44 & 96.62 & 79.20 \\
    ODIN  & 37.33 & 48.27 & 69.80 & 48.91 & 80.83 & 87.44 & 96.62 & 79.20 \\
    \md   & 37.33 & 48.27 & 69.80 & 48.91 & 80.83 & 87.44 & 96.62 & 79.20 \\
    \midrule
    GNNSafe & 17.66 & 30.13 & 50.20 & 27.42 & 56.69 & 79.14 & 96.58 & 64.40 \\
    GraphDE & 46.00 & 37.86 & 69.80 & 40.68 & 77.68 & 88.90 & 96.20 & 77.00 \\
    GOOD-D & /     & /     & /     & /     & /     & /     & /     & / \\
    \midrule
    OCGIN & /     & /     & /     & /     & /     & /     & /     & / \\
    OCGTL & /     & /     & /     & /     & /     & /     & /     & / \\
    GLocalKD & /     & /     & /     & /     & /     & /     & /     & / \\
    \midrule
    SGOOD & \textbf{48.66} & \textbf{48.66} & \textbf{71.60} & \textbf{51.82} & 80.33 & \textbf{89.14} & \textbf{96.66} & \textbf{79.40} \\
    \bottomrule
    \end{tabular}%
    }
  \label{tab:acc}%
  \vspace{-8pt}
\end{table}%
