# Supplementary material for: SGOOD: Substructure-enhanced Graph-Level Out-of-Distribution Detection
Source: arXiv:2310.10237 source file (2024-07-18)
Supplement: Supplementary file 2 [file appendix_double.tex]

\newpage
\appendix

\section{Pseudo-code of \algo}\label{apx:algo}
\vspace{-2mm}

We present the pseudo code of \algo for training and testing in Algorithm \ref{algo:train} and \ref{algo:test} respectively.
\vspace{-4mm}

\begin{algorithm}[!h]
\small	
\caption{Pseudo-code of \algo (Training)}\label{algo:train}
	\DontPrintSemicolon
	\SetNoFillComment
 \textbf{Input:} Training dataset $\Din_{tr}=\{(G_i,y_i)\}^n_{i=1}$,  testing set $\Dtest$, weight of the contrastive loss $\alpha$, number of first-stage pretraining epoch $T_{PT}$, number of second-stage fine-tuning epoch $T_{FT}$\\
 \tcp{Super graph construction}
 Construct   super graphs of substructures $\{\mathcal{G}_{i}\}_{i=1}^{n}$ of all $G_{i} \in \Din_{tr}$;\\
 \tcp{First  stage}
 \For {$epoch=1,2,\ldots, T_{PT}$}{Randomly split training graphs $\Din_{tr}$ into batches $\mathcal{B}$ with batch size $B$;\\
    \For {$\{G_{i}\}_{i=1}^{B} \in \mathcal{B}$}{
        \For {$G_{i} \in \{G_{i}\}_{i=1}^{B}$}{
    Obtain augmented super graphs $\widehat{\mathcal{G}}_{i,0}, \widehat{\mathcal{G}}_{i,1}$ by applying  $\mathcal{T}_{0}$ and $\mathcal{T}_{1}$ to $\mathcal{G}_{i}$;\\
    Obtain augmented graphs $\widehat{G}_{i,0}, \widehat{G}_{i,1}$ according to  $\widehat{\mathcal{G}}_{i,0}, \widehat{\mathcal{G}}_{i,1}$;\\
    Calculate $\mathbf{h}_{\widehat{\mathcal{G}}_{i,0}}$ and $\mathbf{h}_{\widehat{\mathcal{G}}_{i,1}}$ using $(\widehat{G}_{i,0}, \widehat{\mathcal{G}}_{i,0})$ and $(\widehat{G}_{i,1}, \widehat{\mathcal{G}}_{i,1})$ by  Eq.\eqref{eq:node_mp}-\eqref{eq:sub_pool};\\
    Obtain $\mathbf{u}_{\widehat{\mathcal{G}}_{i,0}} = \frac{\psi(\mathbf{h}_{\widehat{\mathcal{G}}_{i,0}})}{||\psi(\mathbf{h}_{\widehat{\mathcal{G}}_{i,0}})||}$ and $\mathbf{u}_{\widehat{\mathcal{G}}_{i,1}} = \frac{\psi(\mathbf{h}_{\widehat{\mathcal{G}}_{i,1}})}{||\psi(\mathbf{h}_{\widehat{\mathcal{G}}_{i,1}})||}$ using shared projection head $\psi$ followed by $l_{2}$-normalization;\\}
    Calculate contrastive loss $\mathcal{L}_{CL}$ by Eq.\eqref{eq:lossCL};\\
    Update parameters using mini-batch gradient descent \wrt $\mathcal{L}_{CL}$;\\
    }}
 \tcp{Second stage}
 \For {$epoch=1,2,\ldots, T_{FT}$}{Randomly split training graphs $\Din_{tr}$ into batches $\mathcal{B}$ with batch size $B$;\\
    \For {$\{G_{i}\}_{i=1}^{B} \in \mathcal{B}$}{
        \For {$G_{i} \in \{G_{i}\}_{i=1}^{B}$}{
        Same as Lines 7-10 ;\\
        Calculate $\mathbf{h}_{\mathcal{G}_{i}}$ using $(G_{i}, \mathcal{G}_{i})$ by  Eq.\eqref{eq:node_mp}-\eqref{eq:sub_pool};\\
%    Obtain augmented super graphs $\widehat{\mathcal{G}}_{i,0}, \widehat{\mathcal{G}}_{i,1}$ by applying  $\mathcal{T}_{0}$ and $\mathcal{T}_{1}$ to $\mathcal{G}_{i}$;\\
 %   Obtain augmented graphs $\widehat{G}_{i,0}, \widehat{G}_{i,1}$ according to  $\widehat{\mathcal{G}}_{i,0}, \widehat{\mathcal{G}}_{i,1}$;\\
   % Calculate $\mathbf{h}_{\mathcal{G}_{i}}$, $\mathbf{h}_{\widehat{\mathcal{G}}_{i,0}}$, and $\mathbf{h}_{\widehat{\mathcal{G}}_{i,1}}$ using $(G_{i}, \mathcal{G}_{i})$, $(\widehat{G}_{i,0}, \widehat{\mathcal{G}}_{i,0})$, and $(\widehat{G}_{i,1}, \widehat{\mathcal{G}}_{i,1})$ by  Eq.\eqref{eq:node_mp}-\eqref{eq:sub_pool};\\
    
    %Obtain $\mathbf{u}_{\widehat{\mathcal{G}}_{i,0}} = \frac{\psi(\mathbf{h}_{\widehat{\mathcal{G}}_{i,0}})}{||\psi(\mathbf{h}_{\widehat{\mathcal{G}}_{i,0}})||}$ and $\mathbf{u}_{\widehat{\mathcal{G}}_{i,1}} = \frac{\psi(\mathbf{h}_{\widehat{\mathcal{G}}_{i,1}})}{||\psi(\mathbf{h}_{\widehat{\mathcal{G}}_{i,1}})||}$ using shared projection head $\psi$ followed by $l_{2}$-normalization;\\
    Calculate  prediction logits $\widehat{y}_{i}$ by applying linear transformation on $\mathbf{h}_{\mathcal{G}_{i}}$;\\
    }
    Calculate cross-entropy loss $\mathcal{L}_{CE}$ by Eq.\eqref{eq:lossce};\\    
    Calculate contrastive loss $\mathcal{L}_{CL}$ by Eq.\eqref{eq:lossCL};\\
    Update parameters using mini-batch gradient descent \wrt $\mathcal{L}_{CE}+\alpha \mathcal{L}_{CL}$;\\
    }}
 \tcp{Estimate class centroids and covariance matrix}
  \For {$G_{i} \in \Din_{tr}$}{
    Calculate $\{\mathbf{h}_{v}|v\in {V}_{i}\}$ and $\mathbf{h}_{\mathcal{G}_{i}}$ using $(G_{i}, \mathcal{G}_{i})$ by  Eq.\eqref{eq:node_mp}-\eqref{eq:sub_pool};\\
    Calculate $\mathbf{h}_{G_{i}}=\texttt{\small{READOUT}}(\{\mathbf{h}_{v}|v\in {V}_{i}\})$;\\
    Calculate $\mathbf{z}_{i} = \frac{\texttt{\small{CONCAT}}(\mathbf{h}_{G_{i}},\mathbf{h}_{\mathcal{G}_{i}})}{||\texttt{\small{CONCAT}}(\mathbf{h}_{G_{i}},\mathbf{h}_{\mathcal{G}_{i}})||_{2}}$;
  }
  Calculate estimated class centroids $\{\bm{\mu}_{c}\}_{c=1}^{C}$ 
and covariance matrix $\widehat{ \Sigma}$ by Eq.\eqref{eq:estimated};\\
\end{algorithm}

\begin{algorithm}[t]
\small	
\caption{Pseudo-code of \algo (OOD Detection During Testing)}\label{algo:test}
	\DontPrintSemicolon
	\SetNoFillComment
 \textbf{Input:} The trained \algo model $f$, testing set $\Dtest$, estimated class centroids $\{\bm{\mu}_{c}\}_{c=1}^{C}$ , estimated covariance matrix $\widehat{ \Sigma}$
 %, threshold of OOD score $\lambda$ 
 \\

 \tcp{Testing stage}
 \For{$G_{i}\in \Dtest$}{
 Construct super graph $\mathcal{G}_{i}$;\\
    Calculate $\{\mathbf{h}_{v}|v\in {V}_{i}\}$ and $\mathbf{h}_{\mathcal{G}_{i}}$ using $(G_{i}, \mathcal{G}_{i})$ and $f$ by  Eq.\eqref{eq:node_mp}-\eqref{eq:sub_pool};\\
     Calculate $\mathbf{h}_{G_{i}}=\texttt{\small{READOUT}}(\{\mathbf{h}_{v}|v\in {V}_{i}\})$;\\
    Calculate $\mathbf{z}_{i} = \frac{\texttt{\small{CONCAT}}(\mathbf{h}_{G_{i}},\mathbf{h}_{\mathcal{G}_{i}})}{||\texttt{\small{CONCAT}}(\mathbf{h}_{G_{i}},\mathbf{h}_{\mathcal{G}_{i}})||_{2}}$;\\
    Calculate OOD score $S(G_i)$ by Eq.\eqref{eq:md};\\
    \If{$G_i$ is not OOD based on $S(G_i)$}{
    Perform classification on $G_i$ via  prediction logits $\widehat{y}_{i}$ by applying linear transformation on $\mathbf{h}_{\mathcal{G}_{i}}$;
    }
 }
\end{algorithm}
